# Supplementary material for: Unifying Epidemic Models with Mixtures
Source: arXiv:2201.04960 source file (2022-01-07)
Supplement: Supplementary file 1 [file concentration-proof.tex]

We begin by defining the filtration $\{ \mathcal{F}^1_t \}_{t \geq 1}$ Where $\mathcal{F}^1_t$ is the $\sigma$-algebra generated by $I_1(0; G) \dots, I_1(t; G)$. We may then define the following difference martingale:
\[ D(t; G) = \frac{I_1(t)}{\max\{I_1(t-1), 1\}} - c_1 \beta \gamma^t \mathbf{1}(I_1(t - 1) > 0) \,. \]
We claim that, in the limit as $n_1$ goes to infinity, $D(t; G)$ is a difference martingale with respect to $\mathcal{F}^1_t$. First, note that $D(t; G)$ is $\mathcal{F}^1_t$ measurable. Next, we see
\begin{align*}
    \lim_{n_1 \rightarrow \infty} \E[D(t; G) | \mathcal{F}^1_{t-1}, A_t] &= \lim_{n_1 \rightarrow \infty} \E\left[ \frac{I_1(t)}{\max\{I_1(t-1), 1\}} - c_1 \beta \gamma^t \mathbf{1}(I_1(t - 1) > 0) \vert \mathcal{F}^1_{t-1} , A_t\right] \\
    = \lim_{n_1 \rightarrow \infty} &\frac{1}{\max \{I_1(t-1; G), 1 \} }\left[n_1 - \sum_{k=0}^{t-1} I_1(k; G)\right] \left( \frac{c_1}{n_1} \beta \gamma^t I_1(t-1; G) + o(n_1) \right) \\&\qquad- c_1 \beta \gamma^t \mathbf{1}(I_1(t - 1) > 0) \,.
\end{align*}
Next, we note that for all $n_1$ for which $I_1(t-1; G) = 0$, it is the case that the above is 0, and for all others, the limit as $n_1$ goes to infinity tends toward 0. Hence, for all possible $\sigma$-algebras $\mathcal{F}^1_{t-1}$, the above limit will tend towards 0.

Further, we note that in the limit as $n_1$ tends towards infinity, $D(t; G)$ becomes a conditionally sub-exponential random variable \citep{vershynin2018high} with parameters $(\frac{1}{3(1 - 6^{-1/3}} +c_1 \beta \gamma^t, 1)$. Specifically, we first note
\begin{align*}
   \lim_{n_1 \rightarrow \infty} &\E[e^{\theta I_1(t; G)} \vert \mathcal{F}^1_{t-1}, A_t ] \\
   &= \lim_{n_1 \rightarrow \infty} \left[ \left[1 - (1 - \frac{c_1}{n_1} \beta \gamma^t)^{I_1(t; G)}\right]e^\theta +  (1 - \frac{c_1}{n_1} \beta \gamma^t)^{I_1(t; G)} \right]^{n_1 - \sum_{k=0}^t I_1(k; G)} \,,
\end{align*}
by noting the conditional distribution of $I_1(t; G)$. We then see, taking the limit of the binomial distribution as it converges in distribution to the Poisson distribution,
\begin{align*}
   \lim_{n_1 \rightarrow \infty} &\E[e^{\theta I_1(t; G)} \vert \mathcal{F}^1_{t-1}, A_t ] = e^{c_1 \beta \gamma^t I_1(t-1; G) (e^\theta - 1)} \\
   &\leq e^{\theta c_1 \beta \gamma^t I_1(t-1; G) + \frac{\theta^2}{2} \left(c_1 \beta \gamma^t I_1(t-1; G)\right) (e-1)} \qquad |\theta| < 1 \,.
\end{align*}
The inequality follows by taking the Taylor expansion of $e^\theta$ in the region where $|\theta| < 1$, as
\begin{align*}
   e^\theta - 1 &= \theta + \sum_{j = 2}^\infty  \frac{\theta^j}{j!} \\
   &\leq \theta + \frac{\theta^2}{2} + \sum_{j = 3}^\infty  \frac{\theta^2}{j!} &&(|\theta| < 1 \implies \theta^j < \theta^2 \forall j \geq 3) \\
   &= \theta + \frac{\theta^2}{2} \left(e - 1 \right) \,.
\end{align*}
Hence, it follows that
\begin{align*}
   \lim_{n_1 \rightarrow \infty} &\E[e^{\theta D(t; G)} \vert \mathcal{F}^1_{t-1}, A_t] = \lim_{n_1 \rightarrow \infty} \E[e^{\theta \left(\frac{I_1(t)}{\max\{I_1(t-1), 1\}} - c_1 \beta \gamma^t \mathbf{1}(I_1(t - 1) > 0)\right)} \vert \mathcal{F}^1_{t-1}, A_t ] \\
   &\leq \lim_{n_1 \rightarrow \infty} e^{\frac{\theta^2}{2} (e-1)c \beta \gamma^k I_1(t-1) /  \max\{I_1(t-1), 1 \}^2 } \\
   &\leq e^{\frac{\theta^2}{2} (e-1) c \beta \gamma^k} \,,
\end{align*}
for all $|\theta| < 1$, where the final inequality follows from the fact that $\max\{I_1(t-1), 1 \} \geq 1$ for all $\mathcal{F}^1_{t-1}$. Hence, we see that in the limit $D(t; G)$ is conditionally sub-exponential with parameters $(c_1 \beta \gamma^t (e-1), 1)$, and therefore the sum $\sum_{\tau = 1}^t D(\tau; G)$ is sub-exponential with parameters $((e-1) \sum_{\tau = 1}^t c_1 \beta \gamma^t , 1)$, implying the claim of Proposition \ref{prop:concentration}. 

To show Corollary \ref{cor:concentration}, we first define the following two sets of events:
\begin{align}
    A_{t, \epsilon} &= \left \lbrace I_1(t; G) = 0 \right\rbrace \bigcup \left\lbrace \left\vert \frac{I_1(t; G)}{I_1(t-1; G)} - c \beta \gamma^t\right\vert \geq \epsilon \right\rbrace\\ 
    D_{t, \epsilon} &= \bigcup_{\tau = 1}^t \left \lbrace I_1(\tau; G) = 0 \right\rbrace \bigcup \left\lbrace \left\vert \sum_{\tau = 1}^t \frac{I_1(\tau; G)}{I_1(\tau-1; G)} - c \beta \gamma^\tau \right\vert \geq \epsilon \right\rbrace \,.
\end{align}
Letting $\epsilon_s = c \beta \sum_{\tau = 1}^{s} \epsilon \gamma^s$, We note that the event $\cap_{s = 1}^t A_{s, \epsilon_s - \epsilon_{s-1}}$ is a subset of the event in the claim of the proposition. Further, we have 
\[ \bigcap_{s = 1}^t D_{s, \epsilon_s} \subseteq \bigcap_{s = 1}^t A_{s, \epsilon_s - \epsilon_{s-1}} \,.\]
Hence, the claim follows from the union bound on the probabilities for $D_{s, \epsilon_s}$.
