# Supplementary material for: Unifying Epidemic Models with Mixtures
Source: arXiv:2201.04960 source file (2022-01-07)
Supplement: Supplementary file 2 [file prob-intercommunity-proof.tex]

In order to show a proof of the claim, we rely on the following inequality, which applies to non-negative random variables which take integer values. 
\begin{lemma}
Let $Y$ be an arbitrary non-negative random variable which takes on integer values. Then,
\[ \P(Y \geq 1) \geq \frac{\E[Y]^2}{\E[Y^2]} \,.\]
\end{lemma}
The proof of this claim follows from an application of the Cauchy-Schwarz inequality to the quantity $\E[Y \mathbf{1}_{Y > 0}]$, which is equal to $\E[Y]$ since $Y$ is non-negative \citep{durrett2019probability}.

Hence, in order to apply the above inequality to $Z(t; G)$, we must compute two quantities,
\begin{align*}
    \E[Z(t; G)] &= \sum_{k = 1}^t \E[X(k;G)] \\
    \E[Z(t; G)^2] &=  \sum_{k = 1}^t \E[X(k;G)^2] + 2\sum_{i = 1}^t \sum_{j = i + 1}^{t} \E[X(i;G)X(j; G)] \,.
\end{align*}

As noted above,

\begin{align*}
    \lim_{n_2 \rightarrow \infty} \lim_{n_1 \rightarrow \infty} \E[X(k;G)] &= (c_{12} \beta) (c_1 \beta)^{k-1} \gamma^{k(k-1)/2} \,,
\end{align*}
and similarly, it can be shown
\begin{align*}
    \lim_{n_2 \rightarrow \infty} \lim_{n_1 \rightarrow \infty} \E[X(k;G)^2] &= [(c_{12} \beta) (c_1 \beta)^{k-1} \gamma^{k(k-1)/2}]^2 + (c_{12} \beta) (c_1 \beta)^{k-1} \gamma^{k(k-1)/2} \,.
\end{align*}

The final term remaining to be computed is $\E[X(i; G) X(j; G)]$ for $j > i$. First, we note

\begin{align*}
    \lim_{n_2 \rightarrow \infty} \lim_{n_1 \rightarrow \infty} \E[X(i; G) X(j; G)] &= \lim_{n_2 \rightarrow \infty} \lim_{n_1 \rightarrow \infty}  \E[\E[X(i; G) X(j; G)| I_1(i-1; G) I_1(j-1; G)]] \\
    &= (c_{12} \beta)^2 \gamma^{i-1} \gamma^{j-1} \lim_{n_1 \rightarrow \infty} \E[I_1(i-1; G) I_1(j-1; G)] \,.
\end{align*}

Next, we note $\E[I_1(k+1; G) I_1(k; G)] = \E[\E[I_1(k+1; G)| I_1(k; G)] I_1(k; G)] = c_1\beta \gamma^k \E[I_1(k; G)^2]$ in the limit as $n_1$ tends towards infinity, so inductively we have

\begin{align*}
    \lim_{n_1 \rightarrow \infty} \E[I_1(i-1; G) I_1(j-1; G)] &= (c_1 \beta)^{j-i} \gamma^{\sum_{\tau = i-1}^{j-2} \tau} \lim_{n_1 \rightarrow \infty} \E[I_1(i; G)^2]  \\
    &= (c_1 \beta)^{j-i} \gamma^{\frac{(j-1)(j-2)}{2} - \frac{(i-1)(i-2)}{2}} \lim_{n_1 \rightarrow \infty} \E[I_1(i-1; G)^2] 
\end{align*}

By iterating the recurrence in the second part of Proposition \ref{prop:gaussian}, we note
\begin{align*}
    \lim_{n_1 \rightarrow \infty} \E[I_1(i-1; G)^2] &= (c_1 \beta)^{2(i-1)} \gamma^{(i-1)(i-2)} \left[1 + \sum_{\tau = 0}^{i - 2} \frac{1}{(c_1 \beta)^{\tau + 1} \gamma^{\tau(\tau + 1)}} \right] \,.
\end{align*}

Combining the above statements, we find

\begin{align*}
    \lim_{n_2 \rightarrow \infty} \lim_{n_1 \rightarrow \infty} \E[X(i; G) X(j; G)] &= (c_{12} \beta)^2 \gamma^{i-1} \gamma^{j-1} \times \\
    &\quad (c_1 \beta)^{j-i} \gamma^{\frac{(j-1)(j-2)}{2} - \frac{(i-1)(i-2)}{2}} \times \\
    &\quad  (c_1 \beta)^{2(i-1)} \gamma^{(i-1)(i-2)} \left[1 + \sum_{\tau = 0}^{i - 2} \frac{1}{(c_1 \beta)^{\tau + 1} \gamma^{\tau(\tau + 1)}} \right] \\
    &= (c_{12} \beta)^2 (c_1 \beta)^{j + i - 2} \gamma^{\frac{j(j-1)}{2} + \frac{i(i-1)}{2}}\left[1 + \sum_{\tau = 0}^{i - 2} \frac{1}{(c_1 \beta)^{\tau + 1} \gamma^{\tau(\tau + 1)}} \right] \,.
\end{align*}

Therefore,
\begin{align*}
    &\lim_{n_2 \rightarrow \infty} \lim_{n_1 \rightarrow \infty}\P(Z(t; G) \geq 1) \geq\\ &\left(\sum_{k = 1}^t (c_{12} \beta) (c_1 \beta)^{k-1} \gamma^{k(k-1)/2} \right)^2\times \\&\bigg[\left(\sum_{k = 1}^t [(c_{12} \beta) (c_1 \beta)^{k-1} \gamma^{k(k-1)/2}]^2 + (c_{12} \beta) (c_1 \beta)^{k-1} \gamma^{k(k-1)/2} \right) + \\ &2 \sum_{i = 1}^t \sum_{j = i + 1}^t (c_{12} \beta)^2 (c_1 \beta)^{j + i - 2} \gamma^{\frac{j(j-1)}{2} + \frac{i(i-1)}{2}}\left[1 + \sum_{\tau = 0}^{i - 2} \frac{1}{(c_1 \beta)^{\tau + 1} \gamma^{\tau(\tau + 1)}} \right] \bigg]^{-1} \,,
\end{align*}
or, equivalently, identifying terms of the numerator with those in the denominator, 
\begin{align*}
    \lim_{n_2 \rightarrow \infty} \lim_{n_1 \rightarrow \infty}\P(Z(t; G) \geq 1)& \geq \\\Bigg[1 +  \kappa_t^{-1} +  
     2 \kappa_t^{-2} \sum_{i = 1}^t \sum_{j = i + 1}^t& (c_{12} \beta)^2 (c_1 \beta)^{j + i - 2} \gamma^{\frac{j(j-1)}{2} + \frac{i(i-1)}{2}}\left[ \sum_{\tau = 0}^{i - 2} \frac{1}{(c_1 \beta)^{\tau + 1} \gamma^{\tau(\tau + 1)}} \right] \Bigg]^{-1} \,,
\end{align*}
where $\kappa_t = \sum_{k = 1}^t (c_{12} \beta) (c_1 \beta)^{k-1} \gamma^{k(k-1)/2}$. Moreover, since $\sum_{\tau = 0}^{i - 2} \frac{1}{(c_1 \beta)^{\tau + 1} \gamma^{\tau(\tau + 1)}}$ is upper bounded by a constant independent of $i$ in any regime where the number of cases is at least $1$, and since $\kappa_t$ is increasing, we see that the lower bound above is also increasing in $t$, and will reach a finite positive limit as it is also upper bounded by 1.
