# Supplementary material for: Unifying Epidemic Models with Mixtures
Source: arXiv:2201.04960 source file (2022-01-07)
Supplement: Supplementary file 3 [file community-proof.tex]

First, note:
\begin{align*}
\E[X(t;G)] &= \E[\E[X(t;G) | I(t-1;G)]] \\
&= n_2 \E[1 - (1 - \frac{c_{12}}{n_2}\beta \gamma^{t-1})^{I(t-1;G)}] \\
\implies \liminf_{n_2 \rightarrow \infty}  \liminf_{n_1 \rightarrow \infty}\E[X(t)]  &= c_{12} \liminf_{n_1 \rightarrow \infty} \E[ \beta I(t-1;G) \gamma^{t-1}]  \\
&= c_{12} \beta \gamma^{t-1} \liminf_{n_1 \rightarrow \infty}\E[I(t-1;G)] \\
&= (c_{12} \beta) (c_1 \beta)^{t-1} \gamma^{t(t+1)/2}
\end{align*}
We then see that, for all $t$,
\begin{align*}
\liminf_{n_2 \rightarrow \infty} \liminf_{n_1 \rightarrow \infty} \E[X(0;G) + X(1;G) + \dots + X(t;G) ] \geq \int_{-\infty}^{t-1} c_{12} \beta \gamma^\tau \times (c_1\beta)^\tau \gamma^{\tau(\tau-1)/ 2} d\tau \,.
\end{align*}
Setting the right-hand side of the equation equal to 1, and using the definition of $I_{1,tot}$, we see:
\begin{align*}
\frac{1}{I_{1,tot}} \int_{-\infty}^{t-1} c_{12} \beta \times (c_1\beta)^\tau \gamma^{\tau(\tau-1)/ 2} \gamma^\tau d\tau = \frac{1}{c_{12} \beta} \times \frac{1}{I_{1,tot}} \,.
\end{align*}
The left hand side now corresponds to the density of a Gaussian random variable with variance $- \log \gamma$ and mean $t_{1, max}$, so we may use an inverse Gaussian CDF function and hence conclude
\[ \liminf_{n_2 \rightarrow \infty}  \liminf_{n_1 \rightarrow \infty} t_{I, n_1, n_2} \geq \Phi^{-1} \left( \frac{1}{c_{12} \beta} \times \frac{1}{I_{1, tot}} \right) \times \frac{1}{\sqrt{-\log \gamma}} + t_{1, max} + 1 \,. \]
