# Supplementary material for: Unifying Epidemic Models with Mixtures
Source: arXiv:2201.04960 source file (2022-01-07)
Supplement: Supplementary file 4 [file exp-uncertainty-proof.tex]

First, note the following from the law of iterated expectation.
\begin{align*}
    \lim_{n_1 \rightarrow \infty} \E[I_1 (t'; G) | I_1(t; G)] = (c_1 \beta)^{t' - i} \gamma^{\frac{t'(t'-1)}{2} - \frac{t(t-1)}{2}} I_1(t; G) \,.
\end{align*}

Next, we also note from the recurrence \eqref{eq:cond-square}, 
\begin{align*}
    \lim_{n_1 \rightarrow \infty} \E[I_1 (t'; G)^2 | I_1(t; G)] &= \left( c_1 \beta \right)^{2(t'-t)} \gamma^{t'(t'-1) - t(t-1)} I_1(t; G)^2 + \\
    &~~~I_1(t; G) \sum_{\tau = i}^{t' - 1} \left(c_1 \beta \right)^{3(t' - \tau) - 2} \gamma^{\frac{3t'(t'-1)}{2} - \frac{3(\tau+1) \tau}{2}} 
\end{align*}

Hence, we see
\begin{align*}
    \lim_{n_1 \rightarrow \infty} \textrm{Var}[I_1 (t'; G)^2 | I_1(t; G)] \leq
    &~~~I_1(t; G) \sum_{\tau = t}^{t' - 1} \bigg(\left(c_1 \beta \right)^{(t' - \tau)} \gamma^{\frac{t'(t'-1)}{2} - \frac{(\tau+1) \tau}{2}} \bigg)^3 \,,
\end{align*}
and the claim then follows from Chebyshev's inequality.
