# Supplementary material for: Unifying Epidemic Models with Mixtures
Source: arXiv:2201.04960 source file (2022-01-07)
Supplement: Supplementary file 5 [file gaussian-proof.tex]

Given $I_1(t; G)$ and $I_2(t; G)$, we see that $I_1(t+1; G)$ is a binomial random variable with $n_1 - \sum_{k=0}^t I_1(k; G)$ trials and probability $ 1 - (1 - \frac{c_1}{n_1} \beta \gamma^t)^{I_1(t; G)} (1 - \frac{c_{21}}{n_1} \beta \gamma^t)^{I_2(t; G)}$ of success.
The number of trials comes from the computation of the remaining susceptible population, and the success probability comes the independence assumption on infection probability, noting that $I_1(t;G)$ individuals in community $1$ are infected and $I_2(t;G)$ individuals in community $2$ are infected, and each has some independent probability of infecting each node in community $1$.

Rewriting the success probability, we have:
\begin{align*}
    1 - (1 - \frac{c_1}{n_1} \beta \gamma^t)^{I_1(t; G)} &(1 - \frac{c_{12}}{n_1} \beta \gamma^t)^{I_2(t; G)}  \\
    &= 1 - \left[1 - I_1(t; G) \frac{c_1}{n_1} \beta \gamma^t  + O\left( \frac{1}{n_1^2} \right) \right] \left[1 - I_2(t; G) \frac{c_{21}}{n_1} \beta \gamma^t  + O\left( \frac{1}{n_1^2} \right) \right] \\
    &=  I_1(t; G) \frac{c_1}{n_1} \beta \gamma^t  +  I_2(t; G) \frac{c_{21}}{n_1} \beta \gamma^t  + O\left( \frac{1}{n_1^2} \right) \,.
\end{align*}
The claim follows by multiplying the success probability above by the number of trials, which is equal to $n_1 - \sum_{k = 0}^t I_1(k; G)$.
