# Supplementary material for: Unifying Epidemic Models with Mixtures
Source: arXiv:2201.04960 source file (2022-01-07)
Supplement: Supplementary file 6 [file iterated-gaussian.tex]

Taking an iterated expectation using \eqref{eq:cond-exp}, we find
\begin{align*}
    \E[I_1(t+1; G)~|~ \mathcal{F}_2^t] &= \prod_{k = 0}^t (c_1 \beta \gamma^k) I_1(0; G) ~+ \\
    &\qquad \sum_{k = 1}^t c_{12} \beta \gamma^k I_2(k; G) \prod_{j = k+1}^t (c_{1}\beta  \gamma^j) + O\left( \frac{1}{n_1} \right) \,.
\end{align*}
Noting $I_1(0; G) = 1$, and that $\sum_{j = 1}^n j = \frac{n(n+1)}{2}$, we may simplify the first and second terms as
\begin{align*}
    \E[I_1(t+1; G)~|~ \mathcal{F}_2^t] &= (c_1 \beta)^{t+1} \gamma^{t(t+1) / 2} + \\
    &\qquad \sum_{k = 1}^t c_{12} \beta \gamma^k I_2(k; G) (c_{1}\beta)^{t - (k+1)}  \gamma^{t(t+1)/ 2 - k(k+1)/2}) + O\left( \frac{1}{n_1} \right) \,.
\end{align*}
The claim then follows by noting for any non-negative real number, $a = e^{\log a}$.
