# Supplementary material for: Unifying Epidemic Models with Mixtures
Source: arXiv:2201.04960 source file (2022-01-07)
Supplement: Supplementary file 7 [file supplement.tex]

\documentclass[aoas]{imsart}

%% Packages
\RequirePackage{amsthm,amsmath,amsfonts,amssymb}
\RequirePackage[authoryear]{natbib}
\RequirePackage[colorlinks,citecolor=blue,urlcolor=blue]{hyperref}
\RequirePackage{graphicx}
\RequirePackage[authoryear]{natbib}
\RequirePackage{algorithm}
\RequirePackage[noend]{algorithmic}
\RequirePackage{url}
\RequirePackage[utf8]{inputenc}
\RequirePackage{xcolor}
\RequirePackage{wrapfig}
\RequirePackage{alphalph}
\RequirePackage{caption}
\RequirePackage{subcaption}
\RequirePackage{physics}
\RequirePackage{booktabs}

\newcommand{\algtheorem}{3.1~}

\newcommand{\theorysection}{4~}

\setcounter{equation}{18}

\startlocaldefs
%%%%%%%%%%%%%%%%%%%%%%%%%%%%%%%%%%%%%%%%%%%%%%
%%                                          %%
%% Uncomment next line to change            %%
%% the type of equation numbering           %%
%%                                          %%
%%%%%%%%%%%%%%%%%%%%%%%%%%%%%%%%%%%%%%%%%%%%%%
%\numberwithin{equation}{section}
%%%%%%%%%%%%%%%%%%%%%%%%%%%%%%%%%%%%%%%%%%%%%%
%%                                          %%
%% For Axiom, Claim, Corollary, Hypothezis, %%
%% Lemma, Theorem, Proposition              %%
%% use \theoremstyle{plain}                 %%
%%                                          %%
%%%%%%%%%%%%%%%%%%%%%%%%%%%%%%%%%%%%%%%%%%%%%%
\theoremstyle{plain}

\newtheorem{theorem}{Theorem}[section]
\newtheorem{lemma}[theorem]{Lemma}
\newtheorem{proposition}[theorem]{Proposition}

%%%%%%%%%%%%%%%%%%%%%%%%%%%%%%%%%%%%%%%%%%%%%%
%%                                          %%
%% For Assumption, Definition, Example,     %%
%% Notation, Property, Remark, Fact         %%
%% use \theoremstyle{remark}                %%
%%                                          %%
%%%%%%%%%%%%%%%%%%%%%%%%%%%%%%%%%%%%%%%%%%%%%%
\theoremstyle{remark}
\newtheorem{definition}[theorem]{Definition}

%%%%%%%%%%%%%%%%%%%%%%%%%%%%%%%%%%%%%%%%%%%%%%
%% Please put your definitions here:        %%
%%%%%%%%%%%%%%%%%%%%%%%%%%%%%%%%%%%%%%%%%%%%%%

\endlocaldefs

% \title{Unifying Epidemic Models with Mixtures}

% \author[1]{Arnab Sarker}
% \author[1,3]{Devavrat Shah}
% \author[1,2]{Ali Jadbabaie}
% \affil[1]{Institute for Data, Systems, and Society, MIT}
% \affil[2]{Department of Civil and Environmental Engineering, MIT}
% \affil[3]{Department of Electrical Engineering and Computer Science, MIT}

% \date{May 2021}

\begin{document}
\begin{frontmatter}
\title{Supplementary Material for \\ Unifying Epidemic Models with Mixtures}
%\title{A sample article title with some additional note\thanksref{t1}}
\runtitle{Unifying Epidemic Models with Mixtures}
%\thankstext{T1}{A sample additional note to the title.}

\begin{aug}
%%%%%%%%%%%%%%%%%%%%%%%%%%%%%%%%%%%%%%%%%%%%%%
%%Only one address is permitted per author. %%
%%Only division, organization and e-mail is %%
%%included in the address.                  %%
%%Additional information can be included in %%
%%the Acknowledgments section if necessary. %%
%%%%%%%%%%%%%%%%%%%%%%%%%%%%%%%%%%%%%%%%%%%%%%
\author[A]{\fnms{Arnab} \snm{Sarker}\ead[label=e1, mark]{arnabs@mit.edu}},
\author[A]{\fnms{Ali} \snm{Jadbabaie}\ead[label=e2, mark]{jadbabai@mit.edu}}
\and
\author[A]{\fnms{Devavrat} \snm{Shah}\ead[label=e3, mark]{devavrat@mit.edu}}
%%%%%%%%%%%%%%%%%%%%%%%%%%%%%%%%%%%%%%%%%%%%%%
%% Addresses                                %%
%%%%%%%%%%%%%%%%%%%%%%%%%%%%%%%%%%%%%%%%%%%%%%
\address[A]{Institute for Data, Systems, and Society, MIT \printead{e1}, \printead{e2}, \printead{e3}}
% \address[B]{Department of Civil and Environmental Engineering, MIT  \printead{e2}}
% \address[C]{Department of Electrical Engineering and Computer Science, MIT \printead{e3}}
\end{aug}

\end{frontmatter}

% \section{Introduction}
% \label{s:intro}
% \input{body/introduction}

% \section{Modeling Epidemics}
% \label{s:background}
% \input{body/background}

% \section{Learning Mixtures from Data}
% \label{s:algorithm}
% \input{body/algorithm}

% \section{Generative Basis for Mixtures}
% \label{s:theory}
% \input{body/theory}

% \section{Closed-Loop Interpretation of Gaussian Curves}
% \label{ss:closed-loop}
% \input{body/control}

% % \section{Empirical Analysis of the Mixture Approach}
% % \label{s:empirical}
% % \input{body/empirical}

% % \section{Policy Implications}
% % \label{s:policy}
% % \input{body/policy}

% \section{Conclusions}
% \label{s:conclusions}
% \input{body/conclusions}

\begin{appendix}

\section{Proof of Theorem \algtheorem}
\label{a:alg-proof}
In this section, we provide a justification of Assumption \ref{assumption:midpoint} by showing that a temporal separation condition on the Gaussian components of the mixture will result in a condition which helps to justify Assumption \ref{assumption:midpoint}.
In order to formalize the result, we define the case ratio, denoted $R(t)$.
\begin{definition}[Case Ratio]
When $r = 2$, the \emph{case ratio} $R(t)$ is defined
\[ R(t) = \frac{M_2 e^{-a_2(t-C_2)^2}}{M_1 e^{-a_1(t-C_1)^2}} \,. \]
\end{definition}
If $R(t)$ is close to 1, then the two component Gaussian curves have similar numbers of cases. 
However, if $R(t)$ is close to 0 or significantly larger than 1, then either the first or second outbreak become the ``dominant'' outbreak, respectively. 
With this quantity defined, the result can then be stated as follows

\begin{proposition} \label{prop:alg_midpoint}
Suppose the parameters of the underlying mixture satisfy
\begin{equation}
    |C_1 - C_2| \geq 
    \frac{1}{2 a_1} \log \left(  \frac{4\left(\frac{1+B}{1-B}\right)^4(1+\epsilon^2) - 2}{1 - 4 \left(\frac{1+B}{1-B}\right)^4 \epsilon} \right) \,,
\end{equation}
for some parameter $0 \leq \epsilon \leq \frac{1}{4} \left( \frac{1-B}{1+B}\right)^4$, when $a_1 = a_2$, or that the parameters satisfy
\begin{align*}
    &|C_1 - C_2| \geq
    &\sqrt{\frac{1}{a_1 a_2}\left(\left(\frac{1}{2}\log \frac{4\left(\frac{1+B}{1-B}\right)^4 [\max\{e^{a_2 - a_1}, e^{a_1 - a_2}\} + \epsilon] - e^{a_2 - a_1} + e^{a_1 - a_2}}{1 - 4 \left(\frac{1+B}{1-B}\right)^4 \sqrt{\epsilon}}\right)^2 + (a_2 - a_1) \log \frac{M_1}{M_2}\right)} \,.
\end{align*}
for  $0 \leq \epsilon \leq \frac{1}{16} \left( \frac{1-B}{1+B}\right)^8$
Then, $t^* = \textrm{argmax}_{t'} S(t')$, where $S(t)$ is defined as in \eqref{eq:st} satisfies
\begin{align*}
    \epsilon \leq R(t^*) \leq \frac{1}{\epsilon}
\end{align*}
\end{proposition}
This proposition shows that as long as the components are temporally well separated, $x[1]$ computed in Line 2 of Algorithm \ref{alg:initialization} will be such that $R(t)$ and $\frac{1}{R(t)}$ are both bounded away from $0$ by a constant.
This gives confidence in the ability for $x[1]$ to satisfy Assumption \ref{assumption:midpoint}.

To begin, we first relate the quantities $S(t)$ and $R(t)$ to one another, in the following lemma.
\begin{lemma} \label{lem:st-rt}
The following relationship holds between $S(t)$ and the case ratio $R(t)$.
\begin{equation*}
\begin{split}
    S(t) &= - 2 a_1 + \log \left( \left( \frac{1 + (R(t)e^{a_1 - a_2})^2}{(1 + R(t))^2}\right) + \frac{R(t)}{(1 + R(t))^2} \left(\frac{e^{-2a_1(t-C_1)}}{e^{-2a_2(t-C_2)}} + \frac{e^{-2a_2(t-C_2)}}{e^{-2a_1(t-C_1)}} \right) e^{a_1 - a_2}\right)  \newline \\
    &\quad + \log \frac{(1 + \eta_{t+1})(1+\eta_{t-1})}{(1 + \eta_t)^2}
\end{split}
\end{equation*}
\end{lemma}
\begin{proof}
We note
\begin{align*}
    \log N(t) &= \log \left( M_1 e^{-a_1(t-C_1)^2} + M_2 e^{-a_2(t-C_2)^2} \right) \\
    &= \log M_1 e^{-a_1(t-C_1)^2}  + \log \left(1 + R(t) \right) \,,
\end{align*}
which allows us to show that
\begin{align*}
    S(t) &= \log \frac{N(t+1)}{N(t)} - \log \frac{N(t)}{N(t-1)} \nonumber \\
    &= \log M_1 e^{-a_1(t + 1 -C_1)^2}  + \log \left(1 + R(t + 1) \right) \nonumber\\
    &\quad - 2 \left(\log M_1 e^{-a_1(t-C_1)^2}  + \log \left(1 + R(t) \right) \right) \nonumber\\
    &\quad + \log M_1 e^{-a_1(t - 1 -C_1)^2}  + \log \left(1 + R(t - 1) \right) \nonumber\\
    &\quad + \log \frac{(1 + \eta_{t+1})(1+\eta_{t-1})}{(1 + \eta_t)^2}\nonumber\\
    &= \log M_1 e^{-a_1(t -C_1)^2 - 2a_1(t-C_1) - a_1} - 2 \log M_1 e^{-a_1(t-C_1)^2} + \log M_1 e^{-a_1(t -C_1)^2 + 2a_1 (t-C_1) - a_1}   \nonumber\\
    &\quad+ \log \left(1 + R(t + 1) \right) - 2 \log \left(1 + R(t) \right) + \log \left(1 + R(t-1) \right) + \log \frac{(1 + \eta_{t+1})(1+\eta_{t-1})}{(1 + \eta_t)^2} \nonumber\\
    &=  - 2 a_1 +  \log \left(1 + R(t + 1) \right) - 2 \log \left(1 + R(t) \right) + \log \left(1 + R(t-1) \right) + \log \frac{(1 + \eta_{t+1})(1+\eta_{t-1})}{(1 + \eta_t)^2} \nonumber\\
    &=  - 2 a_1 +  \log \left(1 + R(t) \frac{e^{-2a_2(t-C_2) - a_2}}{e^{-2a_1(t-C_1) - a_1}} \right) - 2 \log \left(1 + R(t) \right) + \log \left(1 + R(t) \frac{e^{2a_2(t-C_2) - a_2}}{e^{2a_1(t-C_1) - a_1}}\right)\nonumber\\
    &\quad + \log \frac{(1 + \eta_{t+1})(1+\eta_{t-1})}{(1 + \eta_t)^2} \nonumber\\
    &=  - 2 a_1 +  \log \left(1 + R(t) \frac{e^{-2a_2(t-C_2) - a_2}}{e^{-2a_1(t-C_1) - a_1}} + R(t) \frac{e^{2a_2(t-C_2) - a_2}}{e^{2a_1(t-C_1) - a_1}} + R(t)^2 \frac{e^{-2a_2}}{e^{-2a_1}}\right) - 2 \log \left(1 + R(t) \right)\nonumber\\
    &\quad + \log \frac{(1 + \eta_{t+1})(1+\eta_{t-1})}{(1 + \eta_t)^2} \nonumber\\
    &= - 2 a_1 + \log \left( \left( \frac{1 + (R(t)e^{a_1 - a_2})^2}{(1 + R(t))^2}\right) + \frac{R(t)}{(1 + R(t))^2} \left(\frac{e^{-2a_1(t-C_1)}}{e^{-2a_2(t-C_2)}} + \frac{e^{-2a_2(t-C_2)}}{e^{-2a_1(t-C_1)}} \right) e^{a_1 - a_2}\right) \nonumber\\
    &\quad + \log \frac{(1 + \eta_{t+1})(1+\eta_{t-1})}{(1 + \eta_t)^2}\,.
\end{align*}
\end{proof}
This expression clarifies the relationship between $R(t)$ and $S(t)$.
If we momentarily ignore the contribution of the noise, then we can make the following observations.
When $R(t)$ is near 0, the term within the deterministic logarithm is close to $1$, as the first term within the logarithm is close to $1$ and the second is close to 0, resulting in $S(t) \approx -2a_1$, as the first outbreak is dominant in this case.
When $R(t) \gg 1$, then the first term of the sum within the deterministic logarithm approaches $e^{2(a_1 - a_2)}$ and the second again approaches 0, resulting in $S(t) \approx -2a_2$ as the second outbreak becomes dominant.
Interestingly, when $R(t)$ is close to $1$, the second term within the sum of the logarithm begins to have weight.
Mathematically, this is precisely what relates the spike observed in Figure \ref{fig:idealized_st} to the ratio of cases.

The proof for the case where $a_1 = a_2$ also relies on the following lemma.
\begin{lemma}\label{lem:a1-equal-upper}
Suppose $a_1 = a_2$, and fix $0 < \epsilon \leq 1$.
If $R(t) \leq \epsilon$ or $R(t) \geq \frac{1}{\epsilon}$, then
\[ S(t) \leq -2 a_1 + \log \left(1 + \left(e^{2a_1(C_1 - C_2)} + e^{-2a_1(C_1 - C_2)}\right) \epsilon + \epsilon^2 \right) + 2 \log \left( \frac{1+B}{1-B}\right) \,.\]
\end{lemma}
\begin{proof}
In the case $a_1 = a_2$, we have
\begin{align*}
    S(t) &= - 2 a_1 + \log \left( \left( \frac{1 + R(t)^2}{(1 + R(t))^2}\right) + \frac{R(t)}{(1 + R(t))^2} \left(e^{2a_1(C_1 - C_2)} + e^{-2a_1(C_1 - C_2)} \right) \right) \\
    &\qquad + \log \frac{(1 + \eta_{t+1})(1+\eta_{t-1})}{(1 + \eta_t)^2} \\
    &\leq  - 2 a_1 + \log \left( \left( \frac{1 + R(t)^2}{(1 + R(t))^2}\right) + \frac{R(t)}{(1 + R(t))^2} \left(e^{2a_1(C_1 - C_2)} + e^{-2a_1(C_1 - C_2)} \right) \right) \\
    &\qquad +  2 \log \left( \frac{1+B}{1-B}\right) \,,
\end{align*}
where the last expression comes from the boundedness of the noise $\eta_t$. 
Here, we note that the term 
\[ \left( \frac{1 + R(t)^2}{(1 + R(t))^2}\right) + \frac{R(t)}{(1 + R(t))^2} \left(e^{2a_1(C_1 - C_2)} + e^{-2a_1(C_1 - C_2)} \right) \]
is invariant to an inversion of $R(t)$. That is, for $0 < \epsilon \leq 1$, any inequalities on this term that utilize the condition $0 < R(t) \leq \epsilon$ will also hold under the condition $\frac{1}{\epsilon} \leq R(t) < \infty$.

Hence, if $R(t)\leq \epsilon$, then since $0 < R(t) \leq \epsilon$, we have
\begin{align*}
    S(t) &\leq - 2 a_1 + \log \left( \left( \frac{1 + R(t)^2}{(1 + R(t))^2}\right) + \frac{R(t)}{(1 + R(t))^2} \left(e^{2a_1(C_1 - C_2)} + e^{-2a_1(C_1 - C_2)} \right) \right) + 2 \log \left( \frac{1+B}{1-B}\right) \\
    &\leq - 2a_1 + \log \left( \left( 1 + R(t)^2 \right) + R(t) \left(e^{2a_1(C_1 - C_2)} + e^{-2a_1(C_1 - C_2)} \right) \right) + 2 \log \left( \frac{1+B}{1-B}\right) \\
    &\leq - 2 a_1 + \log \left(1 + \left(e^{2a_1(C_1 - C_2)} + e^{-2a_1(C_1 - C_2)}\right) \epsilon + \epsilon^2 \right) + 2 \log \left( \frac{1+B}{1-B}\right) \,.
\end{align*}
The above inequality must also hold for the case $R(t) \geq \frac{1}{\epsilon}$, as noted previously, hence completing the proof.
\end{proof}

We also have the following Lemma for the case where $a_1 = a_2$.
\begin{lemma} \label{lem:a1-equal-lower}
Suppose $a_1 = a_2$, and let $t_m$ represent the time index at which $R(t_m) = 1$, i.e. $t_m$ represents the midpoint between the two Gaussian components.
Then,
\[ S(t_m) \geq - 2a_1 + \log \left( \frac{2 + e^{2a_1(C_1 - C_2)} + e^{-2a_1(C_1 - C_2)}}{4}\right) - 2 \log \left( \frac{1+B}{1-B}\right) \,. \]
\end{lemma}
\begin{proof}
The statement comes from noting the bound on each $\eta_t$ as well as plugging in $R(t_m) = 1$ and $a_1 = a_2$ into the result of Lemma \ref{lem:st-rt}.
\end{proof}

The above lemmas allow us to prove Proposition \ref{prop:alg_midpoint} in the case $a_1 = a_2$. 
Similarly, we can show the following lemmas which relate to the case where $a_1 \neq a_2$.
First, we make the following observation.
\begin{lemma} \label{lem:a1-unequal}
If $a_1 \neq a_2$, then $S(t)$ can be written directly as a function of $R(t)$, as
\begin{align*}
    S(t) &= - 2 a_1 + \log \bigg( \left( \frac{1 + (R(t)e^{a_1 - a_2})^2}{(1 + R(t))^2}\right) \\
    &\quad + \frac{R(t)}{(1 + R(t))^2} \left(e^{2\sqrt{a_1 a_2 (C_1 - C_2)^2 - (a_2 - a_1)\log \frac{R(t)M_1}{M_2}}} + e^{-2\sqrt{a_1 a_2 (C_1 - C_2)^2 - (a_2 - a_1)\log \frac{R(t)M_1}{M_2}}}\right) e^{a_1 - a_2}\bigg) \\
    &\quad + \log \frac{(1 + \eta_{t+1})(1+\eta_{t-1})}{(1 + \eta_t)^2} \,.
\end{align*}
\end{lemma}
\begin{proof}
We begin by computing a form for $t$ explicitly in terms of $R(t)$, as we know it satisfies the following equation:
\begin{align*}
    \frac{M_2 e^{-a_2(t-C_2)^2}}{M_1 e^{-a_1(t-C_1)^2}} &= R(t) \\
    &\implies -a_2(t-C_2)^2 + a_1(t-C_1)^2 = \log \frac{R(t)M_1}{M_2}
\end{align*}
Rewriting the above as a quadratic equation, we see
\begin{align*}
    t =\frac{-(2a_1 C_1 - 2 a_2 C_2) \pm \sqrt{(2a_1 C_1 - 2 a_2 C_2)^2 - 4(a_2 - a_1)\left( \log \frac{R(t)M_1}{M_2} + a_2 C_2^2 - a_1 C_1^2\right)}}{2(a_2 - a_1)} \,.
\end{align*}
This can be simplified, noting
\begin{align*}
    (2a_1 C_1 - 2 a_2 C_2)^2 &= 4a_1^2 C_1^2 + 4a_2^2 C_2^2 - 8 a_1 a_2 C_1 C_2 \\
    4(a_2 - a_1)\left( \log \frac{M_1}{M_2} + a_2 C_2^2 - a_1 C_1^2\right) &= 4 a_2^2 C_2^2 + 4 a_1^2 C_1^2 - 4 a_1 a_2 C_2^2 - 4 a_1 a_2 C_1^2 + 4(a_2 - a_1)\log \frac{R(t)M_1}{M_2} \,.
\end{align*}
Therefore,
\begin{align*}
    t &= \frac{-(2a_1 C_1 - 2 a_2 C_2) \pm \sqrt{- 8 a_1 a_2 C_1 C_2 - (-4 a_1 a_2 C_1^2 - 4 a_1 a_2 C_2^2 + 4(a_2 - a_1)\log \frac{R(t)M_1}{M_2})}}{2(a_2 - a_1)} \\
    &= \frac{-(2a_1 C_1 - 2 a_2 C_2) \pm 2\sqrt{a_1 a_2 (C_1 - C_2)^2 - (a_2 - a_1)\log \frac{R(t)M_1}{M_2}}}{2(a_2 - a_1)} \,.
\end{align*}

We may take this expression and plug it back into the expression for $S(t)$ from Lemma \ref{lem:st-rt}.
This yields
\begin{align*}
    S(t) &= - 2 a_1 + \log \bigg( \left( \frac{1 + (R(t)e^{a_1 - a_2})^2}{(1 + R(t))^2}\right) \\
    &\quad + \frac{R(t)}{(1 + R(t))^2} \left(e^{2\sqrt{a_1 a_2 (C_1 - C_2)^2 - (a_2 - a_1)\log \frac{R(t)M_1}{M_2}}} + e^{-2\sqrt{a_1 a_2 (C_1 - C_2)^2 - (a_2 - a_1)\log \frac{R(t)M_1}{M_2}}}\right) e^{a_1 - a_2}\bigg) \\
    &\quad + \log \frac{(1 + \eta_{t+1})(1+\eta_{t-1})}{(1 + \eta_t)^2} \,,
\end{align*}
proving the claim.
\end{proof}

This is helpful in showing the next statement, which corresponds to Lemma \ref{lem:a1-equal-upper}, but for the case $a_1 \neq a_2$.
\begin{lemma} \label{lem:a1-unequal-upper}
Suppose $a_1 \neq a_2$, and fix $0 < \epsilon \leq \frac{M_2}{M_1} e^{-16(a_2 - a_1)}$. If $R(t) \leq \epsilon$, then
\begin{align*}
    S(t) &\leq - 2 a_1 + \log \bigg( \max \{1, e^{2(a_1 - a_2)}\} + \sqrt{\epsilon} \left(e^{2\sqrt{a_1 a_2 (C_1 - C_2)^2 - (a_2 - a_1) \log \frac{M_1}{M_2}}} + 1\right) e^{a_1 - a_2}\bigg) + 2 \log \frac{1+B}{1-B}
\end{align*}
When $R(t) \geq \frac{1}{\epsilon}$,
\begin{align*}
    S(t) &\leq - 2 a_1 + \log\bigg( \max \{1, e^{2(a_1 - a_2)}\}+  \epsilon \left(e^{2\sqrt{a_1 a_2 (C_1 - C_2)^2 - (a_2 - a_1)\log \frac{M_1}{M_2}}} + 1\right) e^{a_1 - a_2}\bigg) + 2 \log \frac{1+B}{1-B} \,.
\end{align*}
\end{lemma}
\begin{proof}
From Lemma \ref{lem:a1-unequal}, we know that $S(t)$ may be written as
\begin{align*}
    S(t) &= - 2 a_1 + \log \bigg( \left( \frac{1 + (R(t)e^{a_1 - a_2})^2}{(1 + R(t))^2}\right) \\
    &\quad + \frac{R(t)}{(1 + R(t))^2} \left(e^{2\sqrt{a_1 a_2 (C_1 - C_2)^2 - (a_2 - a_1)\log \frac{R(t)M_1}{M_2}}} + e^{-2\sqrt{a_1 a_2 (C_1 - C_2)^2 - (a_2 - a_1)\log \frac{R(t)M_1}{M_2}}}\right) e^{a_1 - a_2}\bigg) \\
    &\quad + \log \frac{(1 + \eta_{t+1})(1+\eta_{t-1})}{(1 + \eta_t)^2} \\
    &\leq - 2 a_1 + \log \bigg( \left( \frac{1 + (R(t)e^{a_1 - a_2})^2}{(1 + R(t))^2}\right) \\
    &\quad + \frac{R(t)}{(1 + R(t))^2} \left(e^{2\sqrt{a_1 a_2 (C_1 - C_2)^2 - (a_2 - a_1)\log \frac{R(t)M_1}{M_2}}} + e^{-2\sqrt{a_1 a_2 (C_1 - C_2)^2 - (a_2 - a_1)\log \frac{R(t)M_1}{M_2}}}\right) e^{a_1 - a_2}\bigg) \\
    &\quad + 2 \log \frac{1+B}{1-B} \\
    &\leq - 2 a_1 + \log \bigg( \left( \frac{1 + (R(t)e^{a_1 - a_2})^2}{(1 + R(t))^2}\right) \\
    &\quad + \frac{R(t)}{(1 + R(t))^2} \left(e^{2\sqrt{a_1 a_2 (C_1 - C_2)^2 - (a_2 - a_1)\log \frac{R(t)M_1}{M_2}}} + 1\right) e^{a_1 - a_2}\bigg) \\
    &\quad + 2 \log \frac{1+B}{1-B} \qquad (*) \\
    &\leq - 2 a_1 + \log \bigg( \left( \frac{1 + (R(t)e^{a_1 - a_2})^2}{(1 + R(t))^2}\right) \\
    &\quad + \frac{R(t)}{(1 + R(t))^2} \left(e^{2\sqrt{a_1 a_2 (C_1 - C_2)^2 - (a_2 - a_1) \log \frac{M_1}{M_2}}} e^{2\sqrt{- (a_2 - a_1)\log R(t)}} + 1\right) e^{a_1 - a_2}\bigg) \\
    &\quad + 2 \log \frac{1+B}{1-B} \,.
\end{align*}
In the first case, when $R(t) \leq e^{-16(a_2 - a_1)}$, we note
\begin{align*}
    &\log \left(R(t)\right) \leq \left( -16(a_2 - a_1)\right) \\
    &\implies \log \left(R(t) \right) \log \left(R(t) \right)  \geq \left( -16(a_2 - a_1)\right)\left(\log R(t) \frac{M_1}{M_2}\right) \\
    &\implies -\frac{1}{2} \log \frac{R(t)}{} \geq 2 \sqrt{-(a_2 - a_1) \log \frac{R(t) M_1}{M_2}} \\
    &\implies e^{2 \sqrt{-(a_2 - a_1) \log R(t)}} \leq \frac{1}{\sqrt{R(t)}} \,.
\end{align*}
This yields
\begin{align*}
    S(t) &\leq - 2 a_1 + \log \bigg( \max \{1, e^{2(a_1 - a_2)}\} + \sqrt{\epsilon} \left(e^{2\sqrt{a_1 a_2 (C_1 - C_2)^2 - (a_2 - a_1) \log \frac{M_1}{M_2}}} + 1\right) e^{a_1 - a_2}\bigg) + 2 \log \frac{1+B}{1-B} \,,
\end{align*}
since $\left( \frac{1 + (R(t)e^{a_1 - a_2})^2}{(1 + R(t))^2}\right) \leq \max\{1, e^{2(a_1 - a_2)}$.
When $R(t) \geq \frac{1}{\epsilon}$, we instead see more directly that
\begin{align*}
    S(t) &\leq - 2 a_1 + \log \bigg( \left( \frac{1 + (R(t)e^{a_1 - a_2})^2}{(1 + R(t))^2}\right) \\
    &\quad + \frac{R(t)}{(1 + R(t))^2} \left(e^{2\sqrt{a_1 a_2 (C_1 - C_2)^2 - (a_2 - a_1)\log \frac{M_1}{M_2}}} + 1\right) e^{a_1 - a_2}\bigg) \\
    &\quad + 2 \log \frac{1+B}{1-B} \,,
\end{align*}
from the equation noted with $(*)$ above.
Applying the fact that $R(t) \geq \frac{1}{\epsilon}$ then yields, because $R(t) / (1+R(t))^2 \leq 1/R(t)$,
\begin{align*}
    S(t) &\leq - 2 a_1 + \log\bigg(\left( \frac{1 + (R(t)e^{a_1 - a_2})^2}{(1 + R(t))^2}\right) \\
    &\quad + \epsilon \left(e^{2\sqrt{a_1 a_2 (C_1 - C_2)^2 - (a_2 - a_1)\log \frac{M_1}{M_2}}} + 1\right) e^{a_1 - a_2}\bigg) \\
    &\quad + 2 \log \frac{1+B}{1-B} \,.
\end{align*}
Finally, we note that $\left( \frac{1 + (R(t)e^{a_1 - a_2})^2}{(1 + R(t))^2}\right) \leq \max\{1, e^{2(a_1 - a_2)}$, completing the claim.
\end{proof}

We may then show the following Lemma, which corresponds to Lemma \ref{lem:a1-equal-lower} for the case $a_1 \neq a_2$.
\begin{lemma} \label{lem:a1-unequal-lower}
Suppose $a_1 \neq a_2$, and let $t_m$ again represent the time index at which $R(t_m) = 1$, i.e. $t_m$ represents the midpoint between the two Gaussian components.
Then,
\begin{align*}
    S(t_m) &\geq - 2 a_1 + \log \bigg( \left( \frac{1 + e^{2(a_1 - a_2)}}{4}\right) \\
    &\quad + \frac{1}{4} \left(e^{2\sqrt{a_1 a_2 (C_1 - C_2)^2 - (a_2 - a_1)\log \frac{M_1}{M_2}}} + e^{-2\sqrt{a_1 a_2 (C_1 - C_2)^2 - (a_2 - a_1)\log \frac{M_1}{M_2}}}\right) e^{a_1 - a_2}\bigg) \\
    &\quad - 2 \log \left(\frac{1+B}{1-B} \right)  \,.
\end{align*}
\end{lemma}
\begin{proof}
From Lemma \ref{lem:a1-unequal}, we see
\begin{align*}
    S(t_m) &= - 2 a_1 + \log \bigg( \left( \frac{1 + e^{2(a_1 - a_2)}}{4}\right) \\
    &\quad + \frac{1}{4} \left(e^{2\sqrt{a_1 a_2 (C_1 - C_2)^2 - (a_2 - a_1)\log \frac{M_1}{M_2}}} + e^{-2\sqrt{a_1 a_2 (C_1 - C_2)^2 - (a_2 - a_1)\log \frac{M_1}{M_2}}}\right) e^{a_1 - a_2}\bigg) \\
    &\quad + \log \frac{(1 + \eta_{t+1})(1+\eta_{t-1})}{(1 + \eta_t)^2} \,,
\end{align*}
and the claim is completed by noting the bound on the noise $\eta_t$
\end{proof}

The above lemmas allow us to state the proof of the Theorem.
In the presentation of the proof, we make the technical assumption that the point at which $R(t) = 1$ is observed in the data.
While this assumption may not always be the case due to discretization of the observations, we note that the assumption can be relaxed by explicitly providing upper and lower bounds for $S(\textrm{nint}(t))$ in terms of $S(t)$ and model parameters.
We present the proof with the stated assumption as follows.

\begin{proof}
We divide the proof into two cases.
When $a_1 = a_2$, we note that by Lemma \ref{lem:a1-equal-lower}, we have
\[ S(t^*) \geq - 2a_1 + \log \left( \frac{2 + e^{2a_1(C_1 - C_2)} + e^{-2a_1(C_1 - C_2)}}{4}\right) - 2 \log \left( \frac{1+B}{1-B}\right)  \,,\]
since $S(t_m)$ is observed and places a lower bound on $S(t^*)$.
Now, suppose towards contradiction that either $R(t^*) \leq \epsilon$ or $R(t^*) \geq \epsilon$
By Lemma \ref{lem:a1-equal-upper}, it would have to be the case that 
\[ S(t^*) \leq -2 a_1 + \log \left(1 + \left(e^{2a_1(C_1 - C_2)} + e^{-2a_1(C_1 - C_2)}\right) \epsilon + \epsilon^2 \right) + 2 \log \left( \frac{1+B}{1-B}\right) \,.\]
However, since $|C_1 - C_2| \geq \frac{1}{2 a_1} \log \left(  \frac{\left(4\frac{1+B}{1-B}\right)^4(1+\epsilon^2) - 2}{1 - 4 \left(\frac{1+B}{1-B}\right)^4 \epsilon}\right),$ we must have
\begin{align*}
    e^{-2a_1 (C_1 - C_2)} + e^{-2a_1 (C_1 - C_2)} > \frac{\left(4\frac{1+B}{1-B}\right)^4(1+\epsilon^2) - 2}{1 - 4 \left(\frac{1+B}{1-B}\right)^4 \epsilon} \,.
\end{align*}
Rearranging this inequality provides
\begin{align*}
&- 2a_1 + \log \left( \frac{2 + e^{2a_1(C_1 - C_2)} + e^{-2a_1(C_1 - C_2)}}{4}\right) - 2 \log \left( \frac{1+B}{1-B}\right) > \\
&\quad -2 a_1 + \log \left(1 + \left(e^{2a_1(C_1 - C_2)} + e^{-2a_1(C_1 - C_2)}\right) \epsilon + \epsilon^2 \right) + 2 \log \left( \frac{1+B}{1-B}\right) \,,
\end{align*} 
indicating that the previous inequalities on $S(t)$ can not hold simultaneously, a contradiction.
This completes the proof of the case where $a_1 = a_2$.

The case for $a_1 = a_2$ follows similarly.
The condition on $|C_1 - C_2|$, combined with the result of Lemma \ref{lem:a1-equal-lower}, implies that
\begin{align*}
    S(t^*) > - 2 a_1 + \log \bigg( \max \{1, e^{2(a_1 - a_2)}\} + \sqrt{\epsilon} \left(e^{2\sqrt{a_1 a_2 (C_1 - C_2)^2 - (a_2 - a_1) \log \frac{M_1}{M_2}}} + 1\right) e^{a_1 - a_2}\bigg) + 2 \log \frac{1+B}{1-B} \,,
\end{align*}
and that 
\begin{align*}
    S(t^*) > - 2 a_1 + \log \bigg( \max \{1, e^{2(a_1 - a_2)}\} + \epsilon \left(e^{2\sqrt{a_1 a_2 (C_1 - C_2)^2 - (a_2 - a_1) \log \frac{M_1}{M_2}}} + 1\right) e^{a_1 - a_2}\bigg) + 2 \log \frac{1+B}{1-B} \,,
\end{align*}
through algebraic rearrangement. 
This then implies the same contradiction as above, as due to Lemma \ref{lem:a1-equal-upper} it must be the case that $R(t) \geq \epsilon$ and $R(t) \leq \frac{1}{\epsilon}$.
\end{proof}

\section{Proof Details for Section \theorysection}
\label{a:theory}
\input{appendix/theory}

% \section{Proof of Proposition \ref{prop:gaussian}}
% \label{a:gaussian}
% \input{appendix/gaussian-proof}

% \section{Proof of Corollary \ref{cor:gaussian}}
% \label{a:iterated-gaussian}
% \input{appendix/iterated-gaussian}

% % \section{Proof of Corollary \ref{cor:exp-uncertainty}}
% % \label{a:exp-uncertainty}
% % \input{appendix/exp-uncertainty-proof}

% \section{Proof of Proposition \ref{prop:concentration}}
% \label{a:concentration}
% \input{appendix/concentration-proof}

% \section{Proof of Proposition \ref{prop:intercommunity}}
% \label{a:community}
% \input{appendix/community-proof}

% \section{Proof of Proposition \ref{prop:prob-intercommunity}}
% \label{a:prob-intercommunity}
% \input{appendix/prob-intercommunity-proof}

% \section{Details of Empirical Results}
% \label{a:data-processing}
% \input{appendix/data-processing}

\end{appendix}

\bibliographystyle{imsart-nameyear} % Style BST file
\bibliography{main.bib}       % Bibliography file (usually '*.bib')

\end{document}
