# Supplementary material for: Unifying Epidemic Models with Mixtures
Source: arXiv:2201.04960 source file (2022-01-07)
Supplement: Supplementary file 8 [file algorithm-proof.tex]

In this section, we provide a justification of Assumption \ref{assumption:midpoint} by showing that a temporal separation condition on the Gaussian components of the mixture will result in a condition which helps to justify Assumption \ref{assumption:midpoint}.
In order to formalize the result, we define the case ratio, denoted $R(t)$.
\begin{definition}[Case Ratio]
When $r = 2$, the \emph{case ratio} $R(t)$ is defined
\[ R(t) = \frac{M_2 e^{-a_2(t-C_2)^2}}{M_1 e^{-a_1(t-C_1)^2}} \,. \]
\end{definition}
If $R(t)$ is close to 1, then the two component Gaussian curves have similar numbers of cases. 
However, if $R(t)$ is close to 0 or significantly larger than 1, then either the first or second outbreak become the ``dominant'' outbreak, respectively. 
With this quantity defined, the result can then be stated as follows

\begin{proposition} \label{prop:alg_midpoint}
Suppose the parameters of the underlying mixture satisfy
\begin{equation}
    |C_1 - C_2| \geq 
    \frac{1}{2 a_1} \log \left(  \frac{4\left(\frac{1+B}{1-B}\right)^4(1+\epsilon^2) - 2}{1 - 4 \left(\frac{1+B}{1-B}\right)^4 \epsilon} \right) \,,
\end{equation}
for some parameter $0 \leq \epsilon \leq \frac{1}{4} \left( \frac{1-B}{1+B}\right)^4$, when $a_1 = a_2$, or that the parameters satisfy
\begin{align*}
    &|C_1 - C_2| \geq
    &\sqrt{\frac{1}{a_1 a_2}\left(\left(\frac{1}{2}\log \frac{4\left(\frac{1+B}{1-B}\right)^4 [\max\{e^{a_2 - a_1}, e^{a_1 - a_2}\} + \epsilon] - e^{a_2 - a_1} + e^{a_1 - a_2}}{1 - 4 \left(\frac{1+B}{1-B}\right)^4 \sqrt{\epsilon}}\right)^2 + (a_2 - a_1) \log \frac{M_1}{M_2}\right)} \,.
\end{align*}
for  $0 \leq \epsilon \leq \frac{1}{16} \left( \frac{1-B}{1+B}\right)^8$
Then, $t^* = \textrm{argmax}_{t'} S(t')$, where $S(t)$ is defined as in \eqref{eq:st} satisfies
\begin{align*}
    \epsilon \leq R(t^*) \leq \frac{1}{\epsilon}
\end{align*}
\end{proposition}
This proposition shows that as long as the components are temporally well separated, $x[1]$ computed in Line 2 of Algorithm \ref{alg:initialization} will be such that $R(t)$ and $\frac{1}{R(t)}$ are both bounded away from $0$ by a constant.
This gives confidence in the ability for $x[1]$ to satisfy Assumption \ref{assumption:midpoint}.


To begin, we first relate the quantities $S(t)$ and $R(t)$ to one another, in the following lemma.
\begin{lemma} \label{lem:st-rt}
The following relationship holds between $S(t)$ and the case ratio $R(t)$.
\begin{equation*}
\begin{split}
    S(t) &= - 2 a_1 + \log \left( \left( \frac{1 + (R(t)e^{a_1 - a_2})^2}{(1 + R(t))^2}\right) + \frac{R(t)}{(1 + R(t))^2} \left(\frac{e^{-2a_1(t-C_1)}}{e^{-2a_2(t-C_2)}} + \frac{e^{-2a_2(t-C_2)}}{e^{-2a_1(t-C_1)}} \right) e^{a_1 - a_2}\right)  \newline \\
    &\quad + \log \frac{(1 + \eta_{t+1})(1+\eta_{t-1})}{(1 + \eta_t)^2}
\end{split}
\end{equation*}
\end{lemma}
\begin{proof}
We note
\begin{align*}
    \log N(t) &= \log \left( M_1 e^{-a_1(t-C_1)^2} + M_2 e^{-a_2(t-C_2)^2} \right) \\
    &= \log M_1 e^{-a_1(t-C_1)^2}  + \log \left(1 + R(t) \right) \,,
\end{align*}
which allows us to show that
\begin{align*}
    S(t) &= \log \frac{N(t+1)}{N(t)} - \log \frac{N(t)}{N(t-1)} \nonumber \\
    &= \log M_1 e^{-a_1(t + 1 -C_1)^2}  + \log \left(1 + R(t + 1) \right) \nonumber\\
    &\quad - 2 \left(\log M_1 e^{-a_1(t-C_1)^2}  + \log \left(1 + R(t) \right) \right) \nonumber\\
    &\quad + \log M_1 e^{-a_1(t - 1 -C_1)^2}  + \log \left(1 + R(t - 1) \right) \nonumber\\
    &\quad + \log \frac{(1 + \eta_{t+1})(1+\eta_{t-1})}{(1 + \eta_t)^2}\nonumber\\
    &= \log M_1 e^{-a_1(t -C_1)^2 - 2a_1(t-C_1) - a_1} - 2 \log M_1 e^{-a_1(t-C_1)^2} + \log M_1 e^{-a_1(t -C_1)^2 + 2a_1 (t-C_1) - a_1}   \nonumber\\
    &\quad+ \log \left(1 + R(t + 1) \right) - 2 \log \left(1 + R(t) \right) + \log \left(1 + R(t-1) \right) + \log \frac{(1 + \eta_{t+1})(1+\eta_{t-1})}{(1 + \eta_t)^2} \nonumber\\
    &=  - 2 a_1 +  \log \left(1 + R(t + 1) \right) - 2 \log \left(1 + R(t) \right) + \log \left(1 + R(t-1) \right) + \log \frac{(1 + \eta_{t+1})(1+\eta_{t-1})}{(1 + \eta_t)^2} \nonumber\\
    &=  - 2 a_1 +  \log \left(1 + R(t) \frac{e^{-2a_2(t-C_2) - a_2}}{e^{-2a_1(t-C_1) - a_1}} \right) - 2 \log \left(1 + R(t) \right) + \log \left(1 + R(t) \frac{e^{2a_2(t-C_2) - a_2}}{e^{2a_1(t-C_1) - a_1}}\right)\nonumber\\
    &\quad + \log \frac{(1 + \eta_{t+1})(1+\eta_{t-1})}{(1 + \eta_t)^2} \nonumber\\
    &=  - 2 a_1 +  \log \left(1 + R(t) \frac{e^{-2a_2(t-C_2) - a_2}}{e^{-2a_1(t-C_1) - a_1}} + R(t) \frac{e^{2a_2(t-C_2) - a_2}}{e^{2a_1(t-C_1) - a_1}} + R(t)^2 \frac{e^{-2a_2}}{e^{-2a_1}}\right) - 2 \log \left(1 + R(t) \right)\nonumber\\
    &\quad + \log \frac{(1 + \eta_{t+1})(1+\eta_{t-1})}{(1 + \eta_t)^2} \nonumber\\
    &= - 2 a_1 + \log \left( \left( \frac{1 + (R(t)e^{a_1 - a_2})^2}{(1 + R(t))^2}\right) + \frac{R(t)}{(1 + R(t))^2} \left(\frac{e^{-2a_1(t-C_1)}}{e^{-2a_2(t-C_2)}} + \frac{e^{-2a_2(t-C_2)}}{e^{-2a_1(t-C_1)}} \right) e^{a_1 - a_2}\right) \nonumber\\
    &\quad + \log \frac{(1 + \eta_{t+1})(1+\eta_{t-1})}{(1 + \eta_t)^2}\,.
\end{align*}
\end{proof}
This expression clarifies the relationship between $R(t)$ and $S(t)$.
If we momentarily ignore the contribution of the noise, then we can make the following observations.
When $R(t)$ is near 0, the term within the deterministic logarithm is close to $1$, as the first term within the logarithm is close to $1$ and the second is close to 0, resulting in $S(t) \approx -2a_1$, as the first outbreak is dominant in this case.
When $R(t) \gg 1$, then the first term of the sum within the deterministic logarithm approaches $e^{2(a_1 - a_2)}$ and the second again approaches 0, resulting in $S(t) \approx -2a_2$ as the second outbreak becomes dominant.
Interestingly, when $R(t)$ is close to $1$, the second term within the sum of the logarithm begins to have weight.
Mathematically, this is precisely what relates the spike observed in Figure \ref{fig:idealized_st} to the ratio of cases.

The proof for the case where $a_1 = a_2$ also relies on the following lemma.
\begin{lemma}\label{lem:a1-equal-upper}
Suppose $a_1 = a_2$, and fix $0 < \epsilon \leq 1$.
If $R(t) \leq \epsilon$ or $R(t) \geq \frac{1}{\epsilon}$, then
\[ S(t) \leq -2 a_1 + \log \left(1 + \left(e^{2a_1(C_1 - C_2)} + e^{-2a_1(C_1 - C_2)}\right) \epsilon + \epsilon^2 \right) + 2 \log \left( \frac{1+B}{1-B}\right) \,.\]
\end{lemma}
\begin{proof}
In the case $a_1 = a_2$, we have
\begin{align*}
    S(t) &= - 2 a_1 + \log \left( \left( \frac{1 + R(t)^2}{(1 + R(t))^2}\right) + \frac{R(t)}{(1 + R(t))^2} \left(e^{2a_1(C_1 - C_2)} + e^{-2a_1(C_1 - C_2)} \right) \right) \\
    &\qquad + \log \frac{(1 + \eta_{t+1})(1+\eta_{t-1})}{(1 + \eta_t)^2} \\
    &\leq  - 2 a_1 + \log \left( \left( \frac{1 + R(t)^2}{(1 + R(t))^2}\right) + \frac{R(t)}{(1 + R(t))^2} \left(e^{2a_1(C_1 - C_2)} + e^{-2a_1(C_1 - C_2)} \right) \right) \\
    &\qquad +  2 \log \left( \frac{1+B}{1-B}\right) \,,
\end{align*}
where the last expression comes from the boundedness of the noise $\eta_t$. 
Here, we note that the term 
\[ \left( \frac{1 + R(t)^2}{(1 + R(t))^2}\right) + \frac{R(t)}{(1 + R(t))^2} \left(e^{2a_1(C_1 - C_2)} + e^{-2a_1(C_1 - C_2)} \right) \]
is invariant to an inversion of $R(t)$. That is, for $0 < \epsilon \leq 1$, any inequalities on this term that utilize the condition $0 < R(t) \leq \epsilon$ will also hold under the condition $\frac{1}{\epsilon} \leq R(t) < \infty$.

Hence, if $R(t)\leq \epsilon$, then since $0 < R(t) \leq \epsilon$, we have
\begin{align*}
    S(t) &\leq - 2 a_1 + \log \left( \left( \frac{1 + R(t)^2}{(1 + R(t))^2}\right) + \frac{R(t)}{(1 + R(t))^2} \left(e^{2a_1(C_1 - C_2)} + e^{-2a_1(C_1 - C_2)} \right) \right) + 2 \log \left( \frac{1+B}{1-B}\right) \\
    &\leq - 2a_1 + \log \left( \left( 1 + R(t)^2 \right) + R(t) \left(e^{2a_1(C_1 - C_2)} + e^{-2a_1(C_1 - C_2)} \right) \right) + 2 \log \left( \frac{1+B}{1-B}\right) \\
    &\leq - 2 a_1 + \log \left(1 + \left(e^{2a_1(C_1 - C_2)} + e^{-2a_1(C_1 - C_2)}\right) \epsilon + \epsilon^2 \right) + 2 \log \left( \frac{1+B}{1-B}\right) \,.
\end{align*}
The above inequality must also hold for the case $R(t) \geq \frac{1}{\epsilon}$, as noted previously, hence completing the proof.
\end{proof}

We also have the following Lemma for the case where $a_1 = a_2$.
\begin{lemma} \label{lem:a1-equal-lower}
Suppose $a_1 = a_2$, and let $t_m$ represent the time index at which $R(t_m) = 1$, i.e. $t_m$ represents the midpoint between the two Gaussian components.
Then,
\[ S(t_m) \geq - 2a_1 + \log \left( \frac{2 + e^{2a_1(C_1 - C_2)} + e^{-2a_1(C_1 - C_2)}}{4}\right) - 2 \log \left( \frac{1+B}{1-B}\right) \,. \]
\end{lemma}
\begin{proof}
The statement comes from noting the bound on each $\eta_t$ as well as plugging in $R(t_m) = 1$ and $a_1 = a_2$ into the result of Lemma \ref{lem:st-rt}.
\end{proof}

The above lemmas allow us to prove Proposition \ref{prop:alg_midpoint} in the case $a_1 = a_2$. 
Similarly, we can show the following lemmas which relate to the case where $a_1 \neq a_2$.
First, we make the following observation.
\begin{lemma} \label{lem:a1-unequal}
If $a_1 \neq a_2$, then $S(t)$ can be written directly as a function of $R(t)$, as
\begin{align*}
    S(t) &= - 2 a_1 + \log \bigg( \left( \frac{1 + (R(t)e^{a_1 - a_2})^2}{(1 + R(t))^2}\right) \\
    &\quad + \frac{R(t)}{(1 + R(t))^2} \left(e^{2\sqrt{a_1 a_2 (C_1 - C_2)^2 - (a_2 - a_1)\log \frac{R(t)M_1}{M_2}}} + e^{-2\sqrt{a_1 a_2 (C_1 - C_2)^2 - (a_2 - a_1)\log \frac{R(t)M_1}{M_2}}}\right) e^{a_1 - a_2}\bigg) \\
    &\quad + \log \frac{(1 + \eta_{t+1})(1+\eta_{t-1})}{(1 + \eta_t)^2} \,.
\end{align*}
\end{lemma}
\begin{proof}
We begin by computing a form for $t$ explicitly in terms of $R(t)$, as we know it satisfies the following equation:
\begin{align*}
    \frac{M_2 e^{-a_2(t-C_2)^2}}{M_1 e^{-a_1(t-C_1)^2}} &= R(t) \\
    &\implies -a_2(t-C_2)^2 + a_1(t-C_1)^2 = \log \frac{R(t)M_1}{M_2}
\end{align*}
Rewriting the above as a quadratic equation, we see
\begin{align*}
    t =\frac{-(2a_1 C_1 - 2 a_2 C_2) \pm \sqrt{(2a_1 C_1 - 2 a_2 C_2)^2 - 4(a_2 - a_1)\left( \log \frac{R(t)M_1}{M_2} + a_2 C_2^2 - a_1 C_1^2\right)}}{2(a_2 - a_1)} \,.
\end{align*}
This can be simplified, noting
\begin{align*}
    (2a_1 C_1 - 2 a_2 C_2)^2 &= 4a_1^2 C_1^2 + 4a_2^2 C_2^2 - 8 a_1 a_2 C_1 C_2 \\
    4(a_2 - a_1)\left( \log \frac{M_1}{M_2} + a_2 C_2^2 - a_1 C_1^2\right) &= 4 a_2^2 C_2^2 + 4 a_1^2 C_1^2 - 4 a_1 a_2 C_2^2 - 4 a_1 a_2 C_1^2 + 4(a_2 - a_1)\log \frac{R(t)M_1}{M_2} \,.
\end{align*}
Therefore,
\begin{align*}
    t &= \frac{-(2a_1 C_1 - 2 a_2 C_2) \pm \sqrt{- 8 a_1 a_2 C_1 C_2 - (-4 a_1 a_2 C_1^2 - 4 a_1 a_2 C_2^2 + 4(a_2 - a_1)\log \frac{R(t)M_1}{M_2})}}{2(a_2 - a_1)} \\
    &= \frac{-(2a_1 C_1 - 2 a_2 C_2) \pm 2\sqrt{a_1 a_2 (C_1 - C_2)^2 - (a_2 - a_1)\log \frac{R(t)M_1}{M_2}}}{2(a_2 - a_1)} \,.
\end{align*}

We may take this expression and plug it back into the expression for $S(t)$ from Lemma \ref{lem:st-rt}.
This yields
\begin{align*}
    S(t) &= - 2 a_1 + \log \bigg( \left( \frac{1 + (R(t)e^{a_1 - a_2})^2}{(1 + R(t))^2}\right) \\
    &\quad + \frac{R(t)}{(1 + R(t))^2} \left(e^{2\sqrt{a_1 a_2 (C_1 - C_2)^2 - (a_2 - a_1)\log \frac{R(t)M_1}{M_2}}} + e^{-2\sqrt{a_1 a_2 (C_1 - C_2)^2 - (a_2 - a_1)\log \frac{R(t)M_1}{M_2}}}\right) e^{a_1 - a_2}\bigg) \\
    &\quad + \log \frac{(1 + \eta_{t+1})(1+\eta_{t-1})}{(1 + \eta_t)^2} \,,
\end{align*}
proving the claim.
\end{proof}

This is helpful in showing the next statement, which corresponds to Lemma \ref{lem:a1-equal-upper}, but for the case $a_1 \neq a_2$.
\begin{lemma} \label{lem:a1-unequal-upper}
Suppose $a_1 \neq a_2$, and fix $0 < \epsilon \leq \frac{M_2}{M_1} e^{-16(a_2 - a_1)}$. If $R(t) \leq \epsilon$, then
\begin{align*}
    S(t) &\leq - 2 a_1 + \log \bigg( \max \{1, e^{2(a_1 - a_2)}\} + \sqrt{\epsilon} \left(e^{2\sqrt{a_1 a_2 (C_1 - C_2)^2 - (a_2 - a_1) \log \frac{M_1}{M_2}}} + 1\right) e^{a_1 - a_2}\bigg) + 2 \log \frac{1+B}{1-B}
\end{align*}
When $R(t) \geq \frac{1}{\epsilon}$,
\begin{align*}
    S(t) &\leq - 2 a_1 + \log\bigg( \max \{1, e^{2(a_1 - a_2)}\}+  \epsilon \left(e^{2\sqrt{a_1 a_2 (C_1 - C_2)^2 - (a_2 - a_1)\log \frac{M_1}{M_2}}} + 1\right) e^{a_1 - a_2}\bigg) + 2 \log \frac{1+B}{1-B} \,.
\end{align*}
\end{lemma}
\begin{proof}
From Lemma \ref{lem:a1-unequal}, we know that $S(t)$ may be written as
\begin{align*}
    S(t) &= - 2 a_1 + \log \bigg( \left( \frac{1 + (R(t)e^{a_1 - a_2})^2}{(1 + R(t))^2}\right) \\
    &\quad + \frac{R(t)}{(1 + R(t))^2} \left(e^{2\sqrt{a_1 a_2 (C_1 - C_2)^2 - (a_2 - a_1)\log \frac{R(t)M_1}{M_2}}} + e^{-2\sqrt{a_1 a_2 (C_1 - C_2)^2 - (a_2 - a_1)\log \frac{R(t)M_1}{M_2}}}\right) e^{a_1 - a_2}\bigg) \\
    &\quad + \log \frac{(1 + \eta_{t+1})(1+\eta_{t-1})}{(1 + \eta_t)^2} \\
    &\leq - 2 a_1 + \log \bigg( \left( \frac{1 + (R(t)e^{a_1 - a_2})^2}{(1 + R(t))^2}\right) \\
    &\quad + \frac{R(t)}{(1 + R(t))^2} \left(e^{2\sqrt{a_1 a_2 (C_1 - C_2)^2 - (a_2 - a_1)\log \frac{R(t)M_1}{M_2}}} + e^{-2\sqrt{a_1 a_2 (C_1 - C_2)^2 - (a_2 - a_1)\log \frac{R(t)M_1}{M_2}}}\right) e^{a_1 - a_2}\bigg) \\
    &\quad + 2 \log \frac{1+B}{1-B} \\
    &\leq - 2 a_1 + \log \bigg( \left( \frac{1 + (R(t)e^{a_1 - a_2})^2}{(1 + R(t))^2}\right) \\
    &\quad + \frac{R(t)}{(1 + R(t))^2} \left(e^{2\sqrt{a_1 a_2 (C_1 - C_2)^2 - (a_2 - a_1)\log \frac{R(t)M_1}{M_2}}} + 1\right) e^{a_1 - a_2}\bigg) \\
    &\quad + 2 \log \frac{1+B}{1-B} \qquad (*) \\
    &\leq - 2 a_1 + \log \bigg( \left( \frac{1 + (R(t)e^{a_1 - a_2})^2}{(1 + R(t))^2}\right) \\
    &\quad + \frac{R(t)}{(1 + R(t))^2} \left(e^{2\sqrt{a_1 a_2 (C_1 - C_2)^2 - (a_2 - a_1) \log \frac{M_1}{M_2}}} e^{2\sqrt{- (a_2 - a_1)\log R(t)}} + 1\right) e^{a_1 - a_2}\bigg) \\
    &\quad + 2 \log \frac{1+B}{1-B} \,.
\end{align*}
In the first case, when $R(t) \leq e^{-16(a_2 - a_1)}$, we note
\begin{align*}
    &\log \left(R(t)\right) \leq \left( -16(a_2 - a_1)\right) \\
    &\implies \log \left(R(t) \right) \log \left(R(t) \right)  \geq \left( -16(a_2 - a_1)\right)\left(\log R(t) \frac{M_1}{M_2}\right) \\
    &\implies -\frac{1}{2} \log \frac{R(t)}{} \geq 2 \sqrt{-(a_2 - a_1) \log \frac{R(t) M_1}{M_2}} \\
    &\implies e^{2 \sqrt{-(a_2 - a_1) \log R(t)}} \leq \frac{1}{\sqrt{R(t)}} \,.
\end{align*}
This yields
\begin{align*}
    S(t) &\leq - 2 a_1 + \log \bigg( \max \{1, e^{2(a_1 - a_2)}\} + \sqrt{\epsilon} \left(e^{2\sqrt{a_1 a_2 (C_1 - C_2)^2 - (a_2 - a_1) \log \frac{M_1}{M_2}}} + 1\right) e^{a_1 - a_2}\bigg) + 2 \log \frac{1+B}{1-B} \,,
\end{align*}
since $\left( \frac{1 + (R(t)e^{a_1 - a_2})^2}{(1 + R(t))^2}\right) \leq \max\{1, e^{2(a_1 - a_2)}$.
When $R(t) \geq \frac{1}{\epsilon}$, we instead see more directly that
\begin{align*}
    S(t) &\leq - 2 a_1 + \log \bigg( \left( \frac{1 + (R(t)e^{a_1 - a_2})^2}{(1 + R(t))^2}\right) \\
    &\quad + \frac{R(t)}{(1 + R(t))^2} \left(e^{2\sqrt{a_1 a_2 (C_1 - C_2)^2 - (a_2 - a_1)\log \frac{M_1}{M_2}}} + 1\right) e^{a_1 - a_2}\bigg) \\
    &\quad + 2 \log \frac{1+B}{1-B} \,,
\end{align*}
from the equation noted with $(*)$ above.
Applying the fact that $R(t) \geq \frac{1}{\epsilon}$ then yields, because $R(t) / (1+R(t))^2 \leq 1/R(t)$,
\begin{align*}
    S(t) &\leq - 2 a_1 + \log\bigg(\left( \frac{1 + (R(t)e^{a_1 - a_2})^2}{(1 + R(t))^2}\right) \\
    &\quad + \epsilon \left(e^{2\sqrt{a_1 a_2 (C_1 - C_2)^2 - (a_2 - a_1)\log \frac{M_1}{M_2}}} + 1\right) e^{a_1 - a_2}\bigg) \\
    &\quad + 2 \log \frac{1+B}{1-B} \,.
\end{align*}
Finally, we note that $\left( \frac{1 + (R(t)e^{a_1 - a_2})^2}{(1 + R(t))^2}\right) \leq \max\{1, e^{2(a_1 - a_2)}$, completing the claim.
\end{proof}


We may then show the following Lemma, which corresponds to Lemma \ref{lem:a1-equal-lower} for the case $a_1 \neq a_2$.
\begin{lemma} \label{lem:a1-unequal-lower}
Suppose $a_1 \neq a_2$, and let $t_m$ again represent the time index at which $R(t_m) = 1$, i.e. $t_m$ represents the midpoint between the two Gaussian components.
Then,
\begin{align*}
    S(t_m) &\geq - 2 a_1 + \log \bigg( \left( \frac{1 + e^{2(a_1 - a_2)}}{4}\right) \\
    &\quad + \frac{1}{4} \left(e^{2\sqrt{a_1 a_2 (C_1 - C_2)^2 - (a_2 - a_1)\log \frac{M_1}{M_2}}} + e^{-2\sqrt{a_1 a_2 (C_1 - C_2)^2 - (a_2 - a_1)\log \frac{M_1}{M_2}}}\right) e^{a_1 - a_2}\bigg) \\
    &\quad - 2 \log \left(\frac{1+B}{1-B} \right)  \,.
\end{align*}
\end{lemma}
\begin{proof}
From Lemma \ref{lem:a1-unequal}, we see
\begin{align*}
    S(t_m) &= - 2 a_1 + \log \bigg( \left( \frac{1 + e^{2(a_1 - a_2)}}{4}\right) \\
    &\quad + \frac{1}{4} \left(e^{2\sqrt{a_1 a_2 (C_1 - C_2)^2 - (a_2 - a_1)\log \frac{M_1}{M_2}}} + e^{-2\sqrt{a_1 a_2 (C_1 - C_2)^2 - (a_2 - a_1)\log \frac{M_1}{M_2}}}\right) e^{a_1 - a_2}\bigg) \\
    &\quad + \log \frac{(1 + \eta_{t+1})(1+\eta_{t-1})}{(1 + \eta_t)^2} \,,
\end{align*}
and the claim is completed by noting the bound on the noise $\eta_t$
\end{proof}

The above lemmas allow us to state the proof of the Theorem.
In the presentation of the proof, we make the technical assumption that the point at which $R(t) = 1$ is observed in the data.
While this assumption may not always be the case due to discretization of the observations, we note that the assumption can be relaxed by explicitly providing upper and lower bounds for $S(\textrm{nint}(t))$ in terms of $S(t)$ and model parameters.
We present the proof with the stated assumption as follows.

\begin{proof}
We divide the proof into two cases.
When $a_1 = a_2$, we note that by Lemma \ref{lem:a1-equal-lower}, we have
\[ S(t^*) \geq - 2a_1 + \log \left( \frac{2 + e^{2a_1(C_1 - C_2)} + e^{-2a_1(C_1 - C_2)}}{4}\right) - 2 \log \left( \frac{1+B}{1-B}\right)  \,,\]
since $S(t_m)$ is observed and places a lower bound on $S(t^*)$.
Now, suppose towards contradiction that either $R(t^*) \leq \epsilon$ or $R(t^*) \geq \epsilon$
By Lemma \ref{lem:a1-equal-upper}, it would have to be the case that 
\[ S(t^*) \leq -2 a_1 + \log \left(1 + \left(e^{2a_1(C_1 - C_2)} + e^{-2a_1(C_1 - C_2)}\right) \epsilon + \epsilon^2 \right) + 2 \log \left( \frac{1+B}{1-B}\right) \,.\]
However, since $|C_1 - C_2| \geq \frac{1}{2 a_1} \log \left(  \frac{\left(4\frac{1+B}{1-B}\right)^4(1+\epsilon^2) - 2}{1 - 4 \left(\frac{1+B}{1-B}\right)^4 \epsilon}\right),$ we must have
\begin{align*}
    e^{-2a_1 (C_1 - C_2)} + e^{-2a_1 (C_1 - C_2)} > \frac{\left(4\frac{1+B}{1-B}\right)^4(1+\epsilon^2) - 2}{1 - 4 \left(\frac{1+B}{1-B}\right)^4 \epsilon} \,.
\end{align*}
Rearranging this inequality provides
\begin{align*}
&- 2a_1 + \log \left( \frac{2 + e^{2a_1(C_1 - C_2)} + e^{-2a_1(C_1 - C_2)}}{4}\right) - 2 \log \left( \frac{1+B}{1-B}\right) > \\
&\quad -2 a_1 + \log \left(1 + \left(e^{2a_1(C_1 - C_2)} + e^{-2a_1(C_1 - C_2)}\right) \epsilon + \epsilon^2 \right) + 2 \log \left( \frac{1+B}{1-B}\right) \,,
\end{align*} 
indicating that the previous inequalities on $S(t)$ can not hold simultaneously, a contradiction.
This completes the proof of the case where $a_1 = a_2$.

The case for $a_1 = a_2$ follows similarly.
The condition on $|C_1 - C_2|$, combined with the result of Lemma \ref{lem:a1-equal-lower}, implies that
\begin{align*}
    S(t^*) > - 2 a_1 + \log \bigg( \max \{1, e^{2(a_1 - a_2)}\} + \sqrt{\epsilon} \left(e^{2\sqrt{a_1 a_2 (C_1 - C_2)^2 - (a_2 - a_1) \log \frac{M_1}{M_2}}} + 1\right) e^{a_1 - a_2}\bigg) + 2 \log \frac{1+B}{1-B} \,,
\end{align*}
and that 
\begin{align*}
    S(t^*) > - 2 a_1 + \log \bigg( \max \{1, e^{2(a_1 - a_2)}\} + \epsilon \left(e^{2\sqrt{a_1 a_2 (C_1 - C_2)^2 - (a_2 - a_1) \log \frac{M_1}{M_2}}} + 1\right) e^{a_1 - a_2}\bigg) + 2 \log \frac{1+B}{1-B} \,,
\end{align*}
through algebraic rearrangement. 
This then implies the same contradiction as above, as due to Lemma \ref{lem:a1-equal-upper} it must be the case that $R(t) \geq \epsilon$ and $R(t) \leq \frac{1}{\epsilon}$.
\end{proof}
% \begin{lemma}[Lower Bound on Size of Spike]
% \label{lem:peak_high}
% $S(t)$ satisfies the following inequality for all $t$:
% \[ 
% S(t) \geq - 2 \left( \frac{a_1 + a_2}{2} \right) + \log \left( \frac{R(t)}{(1 + R(t))^2} \right) + 2\Big\vert a_2 (t-C_2) - a_1 (t-C_1) \Big\vert- 2 \log \frac{1+B}{1-B}
% \,.\]
% \end{lemma}

% \begin{proof}
% The claim follows from the computations above and noting the boundedness of the noise as well.
% Specifically,
% \begin{align*}
%     S(t) &= - 2 a_1 +\log \bigg( \left( \frac{1 + (R(t)e^{a_1 - a_2})^2}{(1 + R(t))^2}\right) + \frac{R(t)}{(1 + R(t))^2} \left(\frac{e^{-2a_1(t-C_1)}}{e^{-2a_2(t-C_2)}} + \frac{e^{-2a_2(t-C_2)}}{e^{-2a_1(t-C_1)}} \right) &&e^{a_1 - a_2}\bigg) \\
%     &\quad + \log \frac{(1 + \eta_{t+1})(1+\eta_{t-1})}{(1 + \eta_t)^2} &&(\text{From~} \eqref{eq:st-rt}) \\
%     &\geq - 2 a_1 + \log \left( \frac{R(t)}{(1 + R(t))^2}\left(\frac{e^{-2a_1(t-C_1)}}{e^{-2a_2(t-C_2)}} + \frac{e^{-2a_2(t-C_2)}}{e^{-2a_1(t-C_1)}} \right) e^{a_1 - a_2}\right)  \\
%     &\quad + \log \frac{(1 + \eta_{t+1})(1+\eta_{t-1})}{(1 + \eta_t)^2} \\
%     &\geq - 2 a_1 + \log \left( \frac{R(t)}{(1 + R(t))^2}\left(\frac{e^{-2a_1(t-C_1)}}{e^{-2a_2(t-C_2)}} + \frac{e^{-2a_2(t-C_2)}}{e^{-2a_1(t-C_1)}} \right) e^{a_1 - a_2}\right) \\
%     &\quad + 2\log \frac{1+B}{1-B} &&(\eta_t \in [-B, B]) \\
%     &= -2a_1 + (a_1 - a_2) + \log \left( \frac{R(t)}{(1 + R(t))^2} \left(\frac{e^{-2a_1(t-C_1)}}{e^{-2a_2(t-C_2)}} + \frac{e^{-2a_2(t-C_2)}}{e^{-2a_1(t-C_1)}} \right)\right) \\
%     &\quad + 2\log \frac{1+B}{1-B} \\
%     &\geq -a_1 - a_2 + \log \left( \frac{R(t)}{(1 + R(t))^2}\right) + \max \left\lbrace \log  \left(\frac{e^{-2a_1(t-C_1)}}{e^{-2a_2(t-C_2)}} \right), \log  \left(\frac{e^{-2a_2(t-C_2)}}{e^{-2a_1(t-C_1)}} \right) \right\rbrace\\
%     &\quad + 2\log \frac{1+B}{1-B} \\
%     &= - 2 \left( \frac{a_1 + a_2}{2} \right) + \log \left( \frac{R(t)}{(1 + R(t))^2} \right) + 2\Big\vert a_2 (t-C_2) - a_1 (t-C_1) \Big\vert- 2 \log \frac{1+B}{1-B} \,.
% \end{align*}
% Here, the penultimate inequality comes from noting that $\frac{e^{-2a_1(t-C_1)}}{e^{-2a_2(t-C_2)}} + \frac{e^{-2a_2(t-C_2)}}{e^{-2a_1(t-C_1)}}$ is at least as large as each of the individual summands.
% \end{proof}

% We note that the above inequality is useful only if $R(t)$ is close to $1$, as otherwise, when $\frac{R(t)}{(1+R(t))^2}$ is close to 0, which occurs at the extremes of $R(t)$, the bound becomes trivial.
% As we show in the proof of Proposition \ref{prop:alg_midpoint}, when applied to the $t$ such that $R(t) = 1$, the condition provides a valuable lower bound.


% We next show the following result which characterizes the flat portions of the $S(t)$ curve and provides a range for which these curves are flat. Namely, when a single outbreak $k$ is dominating, the value of $S(t)$ is approximately equal to $-2 a_k$, as formalized in the following Lemma.

% \textcolor{red}{There may be something incorrect with the following lemma -- need to check carefully.}

% \begin{lemma}[Upper Bound on Flat Segments]
% \label{lem:low_flat}
% Fix $0 < \epsilon \leq 1$. 
% If $t$ satisfies either
% \[ R(t - 1) + R(t+1) \leq \epsilon \,,\]
% or 
% \[ \frac{1}{R(t - 1)} + \frac{1}{R(t + 1)} \leq  \epsilon \,,\]
% then 
% \[ S(t) \leq \max \{- 2 a_2, - 2 a_1 \} + \log (1 + \epsilon) + 2 \log \left( \frac{1+B}{1-B}\right)\,.\]
% \end{lemma}
% \begin{proof}
% We begin by noting that since $R(t+1) = R(t)\frac{e^{-2a_2(t-C_2) - a_2}}{e^{-2a_1(t-C_1) - a_1}}$ and $R(t-1) = R(t)\frac{e^{2a_2(t-C_2) - a_2}}{e^{2a_1(t-C_1) - a_1}}$, 
% we have
% \begin{align*}
%     R(t - 1) + R(t+1) &= R(t) \left[ \frac{e^{2a_2(t-C_2) - a_2}}{e^{2a_1(t-C_1) - a_1}} + \frac{e^{-2a_2(t-C_2) - a_2}}{e^{-2a_1(t-C_1) - a_1}} \right] \\
%     &= R(t)\left(\frac{e^{-2a_2(t-C_2)}}{e^{-2a_1(t-C_1)}} + \frac{e^{-2a_1(t-C_1)}}{e^{-2a_2(t-C_2)}}\right)e^{a_1 - a_2} \\
%     \frac{1}{R(t - 1)} + \frac{1}{R(t + 1)} &= \frac{1}{R(t)} \left[\frac{e^{2a_1(t-C_1) - a_1}}{e^{2a_2(t-C_2) - a_2}} + \frac{e^{-2a_1(t-C_1) - a_1}}{e^{-2a_2(t-C_2) - a_2}}\right] \\
%     &= \frac{1}{R(t)} \left[\frac{e^{2a_1(t-C_1)}}{e^{2a_2(t-C_2)}} + \frac{e^{-2a_1(t-C_1)}}{e^{-2a_2(t-C_2)}}\right] e^{a_2 - a_1}
% \end{align*}
% the above conditions are equivalent to
% \begin{align}
%   R(t) &\leq \frac{\epsilon}{\left(\frac{e^{-2a_1(t-C_1)}}{e^{-2a_2(t-C_2)}} + \frac{e^{-2a_2(t-C_2)}}{e^{-2a_1(t-C_1)}}\right)e^{a_1 - a_2}} \qquad \text{and} \label{eq:rt-reg}\\
%   R(t) &\geq \left(\frac{\epsilon}{\left(\frac{e^{-2a_1(t-C_1)}}{e^{-2a_2(t-C_2)}} + \frac{e^{-2a_2(t-C_2)}}{e^{-2a_1(t-C_1)}}\right)e^{a_2 - a_1}}\right)^{-1} \label{eq:rt-inv}\,,
% \end{align}
% respectively. We next note that for any constant $\delta > 0$, if $0 \leq R(t) \leq \delta$ or $R(t) \geq 1/\delta$, then $\frac{R(t)}{(1 + R(t))^2} \leq \delta$. The first case follows from the fact that $R(t)$ is non-negative, and the second follows from the fact that $\frac{R(t)}{(1 + R(t))^2} \leq \frac{1}{R(t)}$ for $R(t) > 0$.
% We first show the proof for \eqref{eq:rt-reg}, and see that
% \begin{align*}
%     S(t) &= - 2 a_1 +\log \bigg( \left( \frac{1 + (R(t)e^{a_1 - a_2})^2}{(1 + R(t))^2}\right) + \frac{R(t)}{(1 + R(t))^2} \left(\frac{e^{-2a_1(t-C_1)}}{e^{-2a_2(t-C_2)}} + \frac{e^{-2a_2(t-C_2)}}{e^{-2a_1(t-C_1)}} \right) &&e^{a_1 - a_2}\bigg) \\
%     &\quad + \log \frac{(1 + \eta_{t+1})(1+\eta_{t-1})}{(1 + \eta_t)^2} &&(\text{From~} \eqref{eq:st-rt}) \\
%     &\leq - 2 a_1 + \log \bigg( \left( \frac{1 + (R(t)e^{a_1 - a_2})^2}{(1 + R(t))^2}\right) + \epsilon \bigg)+ 2 \log \left( \frac{1+B}{1-B}\right) \,.
% \end{align*}
% There are then two cases. 
% If $\left( \frac{1 + (R(t)e^{a_1 - a_2})^2}{(1 + R(t))^2}\right) \leq 1$, the claim is immediate. 
% Otherwise, 
% \begin{align*}
%   S(t) &\leq  - 2 a_1 + \log \left( \left( \frac{1 + (R(t)e^{a_1 - a_2})^2}{(1 + R(t))^2}\right) + \epsilon \right) + 2 \log \left( \frac{1+B}{1-B}\right) \\
%   &\leq  - 2 a_1 + \log \left( \left( \frac{1 + (R(t)e^{a_1 - a_2})^2}{(1 + R(t))^2}\right)+ \left( \frac{1 + (R(t)e^{a_1 - a_2})^2}{(1 + R(t))^2}\right) \epsilon \right) + 2 \log \left( \frac{1+B}{1-B}\right) \\
%   &= - 2 a_1 + \log \left( \frac{1 + (R(t)e^{a_1 - a_2})^2}{(1 + R(t))^2} \right) + \log (1 + \epsilon) + 2 \log \left( \frac{1+B}{1-B}\right) \\
%   &\leq - 2 a_1 + \log \left( \frac{(1 + R(t))^2 e^{2(a_1 - a_2)}}{(1 + R(t))^2} \right) + \log (1 + \epsilon) + 2 \log \left( \frac{1+B}{1-B}\right) \\
%   &= - 2 a_2 + \log (1 + \epsilon) + 2 \log \left( \frac{1+B}{1-B}\right) 
% %   &\leq - 2 a_1 + 2\log \left( \frac{e^{a_1 - a_2} + R(t)e^{a_1 - a_2}}{1 + R(t)} \right) + \log (1 + \epsilon) + 2 \log \left( \frac{1+B}{1-B}\right) \\
% %   &\leq - 2 a_1 + 2 \log \left( e^{a_1 - a_2} \right) + \log (1 + \epsilon) + 2 \log \left( \frac{1+B}{1-B}\right)\\
% %   &= - 2 a_2 + \log\left(1 + \epsilon \right) + 2 \log \left( \frac{1+B}{1-B}\right) \,.
% \end{align*}
% The proof for \eqref{eq:rt-inv} follows similarly, as
% \begin{align*}
%     S(t) &= - 2 a_1 +\log \bigg( \left( \frac{1 + R(t)e^{a_1 - a_2}}{1 + R(t)}\right)^2 + \frac{R(t)}{(1 + R(t))^2} \left(\frac{e^{-2a_1(t-C_1)}}{e^{-2a_2(t-C_2)}} + \frac{e^{-2a_2(t-C_2)}}{e^{-2a_1(t-C_1)}} \right) &&e^{a_1 - a_2}\bigg) \\
%     &\quad + \log \frac{(1 + \eta_{t+1})(1+\eta_{t-1})}{(1 + \eta_t)^2} &&(\text{From~} \eqref{eq:st-rt}) \\
%     &\leq - 2 a_1 + \log \bigg( \left( \frac{1 + R(t)e^{a_1 - a_2}}{1 + R(t)}\right)^2 + \epsilon e^{2(a_1 - a_2)}\bigg)+ 2 \log \left( \frac{1+B}{1-B}\right) \,.
% \end{align*}
% If $e^{a_1 - a_2} \leq 1$, the claim is immediate.
% Otherwise, we similarly find 
% \begin{align*}
%   S(t) &\leq  - 2 a_1 + \log \left( \left( \frac{1 + R(t)e^{a_1 - a_2}}{1 + R(t)}\right)^2 + \epsilon e^{2(a_1 - a_2)} \right) + 2 \log \left( \frac{1+B}{1-B}\right) \\
%   &\leq  - 2 a_1 + \log  \left( e^{2(a_1 - a_2)} (1 + \epsilon) \right) + 2 \log \left( \frac{1+B}{1-B}\right) \\
%   &=   - 2 a_2 + \log\left(1 + \epsilon \right) + 2 \log \left( \frac{1+B}{1-B}\right) \,,
% \end{align*}
% completing the proof.
% \end{proof}

% With the above two lemmas, we can combine the results to prove Proposition \ref{prop:alg_midpoint}.
% In the presentation of the proof, we make the technical assumption that the point at which $R(t) = 1$ is observed in the data.
% While this assumption may not always be the case due to discretization of the observations, we note that the assumption can be relaxed by explicitly providing upper and lower bounds for $S(\textrm{nint}(t))$ in terms of $S(t)$ and model parameters.
% We present the proof with the stated assumption as follows.
% \begin{proof}
% Consider the $t$ for which $R(t) = 1$, which we will refer to as $t_m$.
% We may solve for $t_m$ explicitly, as it satisfies
% \[ M_1 e^{-a_1(t_m-C_1)^2} = M_2 e^{-a_2(t_m-C_2)^2} \,,\]
% or equivalently,
% \[ (a_2 - a_1) t_m^2 + (2a_1 C_1 - 2 a_2 C_2) t_m + \log \frac{M_1}{M_2} + a_2 C_2^2 - a_1 C_1^2 = 0 \,.\]
% If $a_1 = a_2$, the expression for $t_m$ is simply
% \[ t_m = \frac{\log \frac{M_1}{M_2} + a_1 (C_2^2 - C_1^2)}{2a_1(C_2 - C_1)} \,. \]
% Otherwise, if $a_1 \neq a_2$, we must solve a quadratic equation to ascertain the value of $t_m$.
% \begin{align*}
%     t_m =\frac{-(2a_1 C_1 - 2 a_2 C_2) \pm \sqrt{(2a_1 C_1 - 2 a_2 C_2)^2 - 4(a_2 - a_1)\left( \log \frac{M_1}{M_2} + a_2 C_2^2 - a_1 C_1^2\right)}}{2(a_2 - a_1)} \,.
% \end{align*}
% This can be simplified, noting
% \begin{align*}
%     (2a_1 C_1 - 2 a_2 C_2)^2 &= 4a_1^2 C_1^2 + 4a_2^2 C_2^2 - 8 a_1 a_2 C_1 C_2 \\
%     4(a_2 - a_1)\left( \log \frac{M_1}{M_2} + a_2 C_2^2 - a_1 C_1^2\right) &= 4 a_2^2 C_2^2 + 4 a_1^2 C_1^2 - 4 a_1 a_2 C_2^2 - 4 a_1 a_2 C_1^2 + 4(a_2 - a_1)\log \frac{M_1}{M_2} \,.
% \end{align*}
% Therefore,
% \begin{align*}
%     t_m &= \frac{-(2a_1 C_1 - 2 a_2 C_2) \pm \sqrt{- 8 a_1 a_2 C_1 C_2 - (-4 a_1 a_2 C_1^2 - 4 a_1 a_2 C_2^2 + 4(a_2 - a_1)\log \frac{M_1}{M_2})}}{2(a_2 - a_1)} \\
%     &= \frac{-(2a_1 C_1 - 2 a_2 C_2) \pm 2\sqrt{a_1 a_2 (C_1 - C_2)^2 - (a_2 - a_1)\log \frac{M_1}{M_2}}}{2(a_2 - a_1)} \,.
% \end{align*}
% Hence, from Lemma \ref{lem:peak_high}, we have the following inequality:
% \begin{align*}
%     S(t_m) &\geq - 2 \left( \frac{a_1 + a_2}{2} \right)  + \log \left( \frac{R(t_m)}{(1 + R(t_m))^2} \right) \\
%     &\quad + 2\Big\vert a_2 (t_m-C_2) - a_1 (t_m-C_1) \Big\vert- 2 \log \frac{1+B}{1-B} \\
%     &= - 2 \left( \frac{a_1 + a_2}{2} \right) - 2 \log 2 + 2\Big\vert a_2 (t_m-C_2) - a_1 (t_m-C_1) \Big\vert- 2 \log \frac{1+B}{1-B} &&(R(t_m) = 1) \\
%     &= - 2 \left( \frac{a_1 + a_2}{2} \right) - 2 \log 2 + \Big\vert 2 (a_2 - a_1) t_m - (2 a_1 C_1 - 2 a_2 C_2) \Big\vert- 2 \log \frac{1+B}{1-B} \,.
% \end{align*}
% There are then two cases.
% If $a_1 = a_2$, the inequality states
% \begin{align*}
%     S(t_m) &\geq - 2 \left( \frac{a_1 + a_2}{2} \right) - 2 \log 2 + 2 a_1 \Big\vert C_2 - C_1 \Big\vert- 2 \log \frac{1+B}{1-B} \,,
% \end{align*}
% and if $a_1 \neq a_2$, it states
% \begin{align*}
%   S(t_m)&\geq - 2 \left( \frac{a_1 + a_2}{2} \right) - 2 \log 2 +  2\sqrt{a_1 a_2 (C_1 - C_2)^2 - (a_2 - a_1)\log \frac{M_1}{M_2}} - 2 \log \frac{1+B}{1-B} \,.
% \end{align*}
% In both cases it is clear that the magnitude of $|C_1 - C_2|$ modulates the size of the lower bound at this specific point in time $t_m$.

% Specifically, plugging in the conditions of Proposition \ref{prop:alg_midpoint}, we find
% \begin{align*}
%   S(t_m)&\geq  \max \{- 2 a_2, - 2 a_1 \} + \log (1 + \delta) + 2 \log \left( \frac{1+B}{1-B}\right) \,.
% \end{align*}
% Since $S(t_m)$ provides a lower bound for $S(t^*)$, as we assume that $S(t_m)$ is an observed quantity, the claim follows from Lemma \ref{lem:low_flat}, as there would otherwise be a contradiction.
% \end{proof}


% Finally, we may combine the results of the two lemmas above in order to show that, under a bounded noise condition, we may approximately identify a point at which the number of cases in each outbreak is comparable, which is shown in Theorem \ref{thm:alg_midpoint}. The proof of this theorem is as follows.

% \begin{proof}
% First, we note that, since the noise is bounded, when $R(t) = 1$, by Lemma \ref{lem:peak_high}, $\tilde{S}(t)$ must satisfy
% \begin{align*}
%     \tilde{S}(t) \geq -2 \left(\frac{a_1 + a_2}{2}\right) + \tau' - 2 \log 2 - W \,,
% \end{align*}
% where $\tau' = \log \left( e^{2\sqrt{a_1 a_2 \tau^2 + (a_2 - a_1) \log \frac{M_2}{M_1}}} - 2 \right)$. By the constraint on $\tau$, this implies
% \[ \tilde{S}(t) \geq - \max \{- 2 a_2, - 2 a_1 \} +  \epsilon + W \,. \]
% This directly implies the claim, as, for $R(t)$ outside the specified range, we must have
% \begin{align*}
%   \tilde{S}(t) &\leq - \max \{- 2 a_2, - 2 a_1 \} + \log (1 + \epsilon) + W  \\
%   &\leq  - \max \{- 2 a_2, - 2 a_1 \} + \epsilon + W \,,
% \end{align*}
% by Lemma \ref{lem:low_flat}, a contradiction.
% \end{proof}


% The above theorem shows that, when the two outbreaks are well separated, $R(t)$ at the value which maximizes $S(t)$ will be close to 1. In this sense, the identified point will be an appropriate separation point at which each individual outbreak should be considered as ``dominating'' the overall time series $N(t)$. It is worth noting that this result may be generalized to the case in which there are $r > 3$ peaks, under the assumption that no more than two outbreaks are non-negligible at any time $t$. Based on the set of assumptions on the size and separation of the different outbreaks, Line 2 of Algorithm \ref{alg:initialization} may be modified appropriately; in practice, we assume that the peaks are separated by at least 60 days and then perform a standard peak finding routine.
